# Supplementary material for: A search for variable subdwarf B stars in TESS Full Frame Images II. Variable objects in the northern ecliptic hemisphere
Source: arXiv:2105.01077 ancillary file (2021-05-03)

**Non-sdB classified variables.**  
**The table is followed by the amplitude spectra or phased time-series of these objects.**

| Gaia DR2                  | TIC        | Spectral Type | G<br>[mag] | Sector         | Period<br>[days] | Remarks                                      |
|---------------------------|------------|---------------|------------|----------------|------------------|----------------------------------------------|
| <b>Pulsators</b>          |            |               |            |                |                  |                                              |
| 1625627602365544832       | 198209459  | B2            | 13.5254    | 14-26          | -                | 2 objects within 21"                         |
| 1713032695100155904       | 298091568  | B4.1          | 15.0012    | 14,15,20,21    | -                | 2 objects within 30"                         |
| 1861191062326013696       | 1955410399 | A0            | 10.3106    | 14,15          | -                | 3 objects within 32"                         |
| 2077737678383889408       | 270610177  | Be            | 11.7726    | 14,15          | -                | <a href="#">Reinhold et al. (2013)</a>       |
| 2132171608553758336       | 279919275  | B3V           | 13.4577    | 14,15,26       | -                | -                                            |
| 2276592430799302912       | 315774160  | B             | 14.5702    | 16-19,24-25    | -                | 3 objects within 32"                         |
| 565004017238715264        | 609754520  | A7IV          | 6.6357     | 18,19,24,26    | -                | -                                            |
| <b>Eclipsing binaries</b> |            |               |            |                |                  |                                              |
| 1821225425253990400       | 209942349  | A3            | 10.4677    | 14             | 1.1762           | very crowded field                           |
| 431584053656962816        | 283020391  | DAB           | 16.2654    | 17,18          | 6.3199           | object 12" away                              |
| 4322472232203849856       | 68975924   | A2            | 9.0130     | 14             | 3.4703           | -                                            |
| <b>Phased lightcurves</b> |            |               |            |                |                  |                                              |
| 1075871822836912128       | 371767486  | DA:           | 15.7809    | 14,20,21       | 0.8906           | -                                            |
| 1152688378078955264       | 459905076  | DA:           | 15.2861    | 25,26          | 0.4294           | -                                            |
| 1459266575345109248       | 950014908  | DA            | 18.9155    | 23             | 0.2015           | -                                            |
| 1533367920984344320       | 18084735   | B4V           | 11.5687    | 22             | 0.5465           | -                                            |
| 1542252151028439808       | 233640529  | A5            | 12.4525    | 22             | 0.4131           | -                                            |
| 1605967612907047808       | 161002462  | B5.7          | 13.4325    | 16,22,23       | 3.2063           | -                                            |
| 1659906934649659136       | 441686959  | B7.4          | 13.2220    | 15,16,22,23    | 1.4122           | -                                            |
| 1828813777784480128       | 395530534  | B8V           | 7.4272     | 14             | 1.3056           | -                                            |
| 733024134288133120        | 82263882   | B6            | 13.5416    | 22             | 1.0151           | -                                            |
| 767386312198060160        | 10113134   | B             | 12.9598    | 22             | 0.9451           | -                                            |
| 2100882501225439488       | 120819719  | B             | 13.4363    | 14             | 1.9043           | <a href="#">Reinhold et al. (2013)</a>       |
| 936051906999100800        | 334276196  | B7            | 15.7925    | 20             | 2.8301           | RS CVn ( <a href="#">Drake et al. 2014</a> ) |
| 747335579498454144        | 173005060  | B             | 14.2143    | 21             | 2.3108           | -                                            |
| <b>Amplitude spectra</b>  |            |               |            |                |                  |                                              |
| 1000850426487401728       | 14196017   | B1            | 14.1613    | 20             | -                | object 9" away                               |
| 1006212675978250240       | 339539154  | B1            | 14.5041    | 19,20          | -                | -                                            |
| 1328057763997734144       | 57158280   | B2p           | 13.1287    | 24,25          | -                | very crowded field                           |
| 1357436478465245184       | 115351563  | B             | 16.0317    | 24,25          | -                | crowded field                                |
| 1511544337452190592       | 332350597  | B9kp          | 11.5628    | 22,23          | -                | -                                            |
| 1662011812222609280       | 1001373800 | B             | 16.8434    | 15,16          | -                | 2 objects within 21"                         |
| 1683580626882189312       | 142961094  | B9.6          | 14.9794    | 14,15,21       | -                | -                                            |
| 1706963459634476928       | 160409651  | B8.7          | 14.7709    | 14-15,19-22,26 | -                | -                                            |
| 1862531534485984256       | 427303386  | A0            | 9.7728     | 14,15          | -                | crowded field                                |
| 1865673736869022848       | 236211659  | B             | 12.1967    | 15             | -                | -                                            |
| 1909071392087590656       | 120598109  | DBA           | 15.0068    | 16             | -                | object 11" away                              |
| 1988623257385378304       | 65989760   | B             | 12.8990    | 16,17          | -                | 4 bright objects within 21"                  |
| 2099876757323090304       | 399792855  | B3V:p         | 11.2097    | 14,26          | -                | -                                            |
| 2106552442170221312       | 279911599  | B             | 16.5875    | 14,26          | -                | <a href="#">Reinhold et al. (2013)</a>       |
| 2130935452546450944       | 299032735  | B             | 13.0351    | 14,15          | -                | <a href="#">Reinhold et al. (2013)</a>       |
| 2131117284281652992       | 399912033  | B             | 14.7895    | 14,15          | -                | <a href="#">Reinhold et al. (2013)</a>       |

|                    |           |        |         |          |   |               |
|--------------------|-----------|--------|---------|----------|---|---------------|
| 300118776907986560 | 5645757   | B      | 11.6710 | 18       | - | -             |
| 426510559099112832 | 605260809 | A2III: | 10.1721 | 17,18,24 | - | crowded field |
| 474298671637654400 | 392371303 | A0     | 10.4433 | 19       | - | crowded field |
| 693490266000488704 | 126318109 | B      | 12.2537 | 21       | - | -             |
| 709613951186153472 | 172933463 | B8     | 10.3411 | 21       | - | -             |
| 791009766199488128 | 11894192  | DA:    | 14.6829 | 22       | - | -             |
| 908509660415660416 | 99010997  | B8     | 10.1411 | 20       | - | -             |

---

### Pulsators

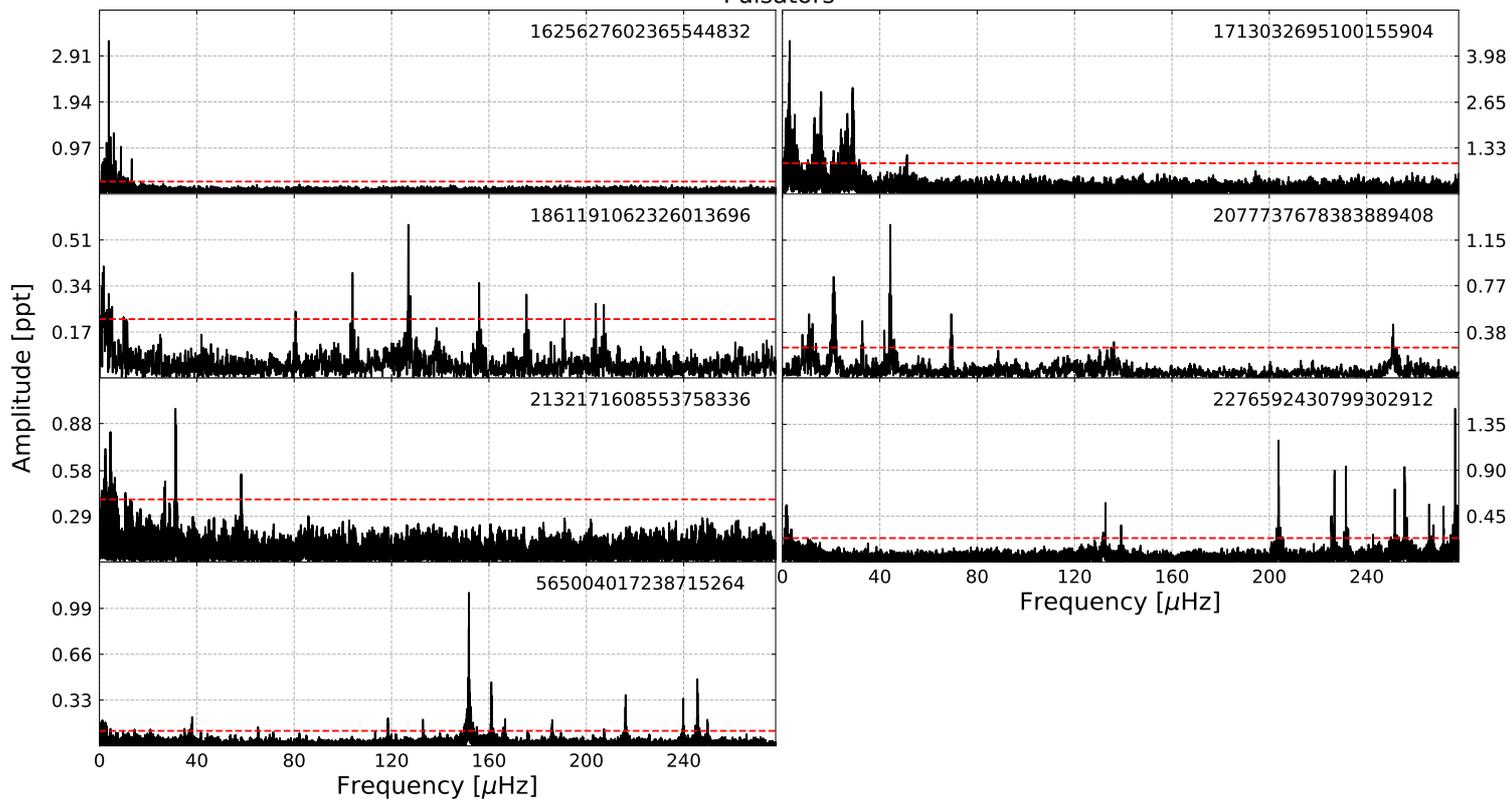

### Eclipsing Binaries

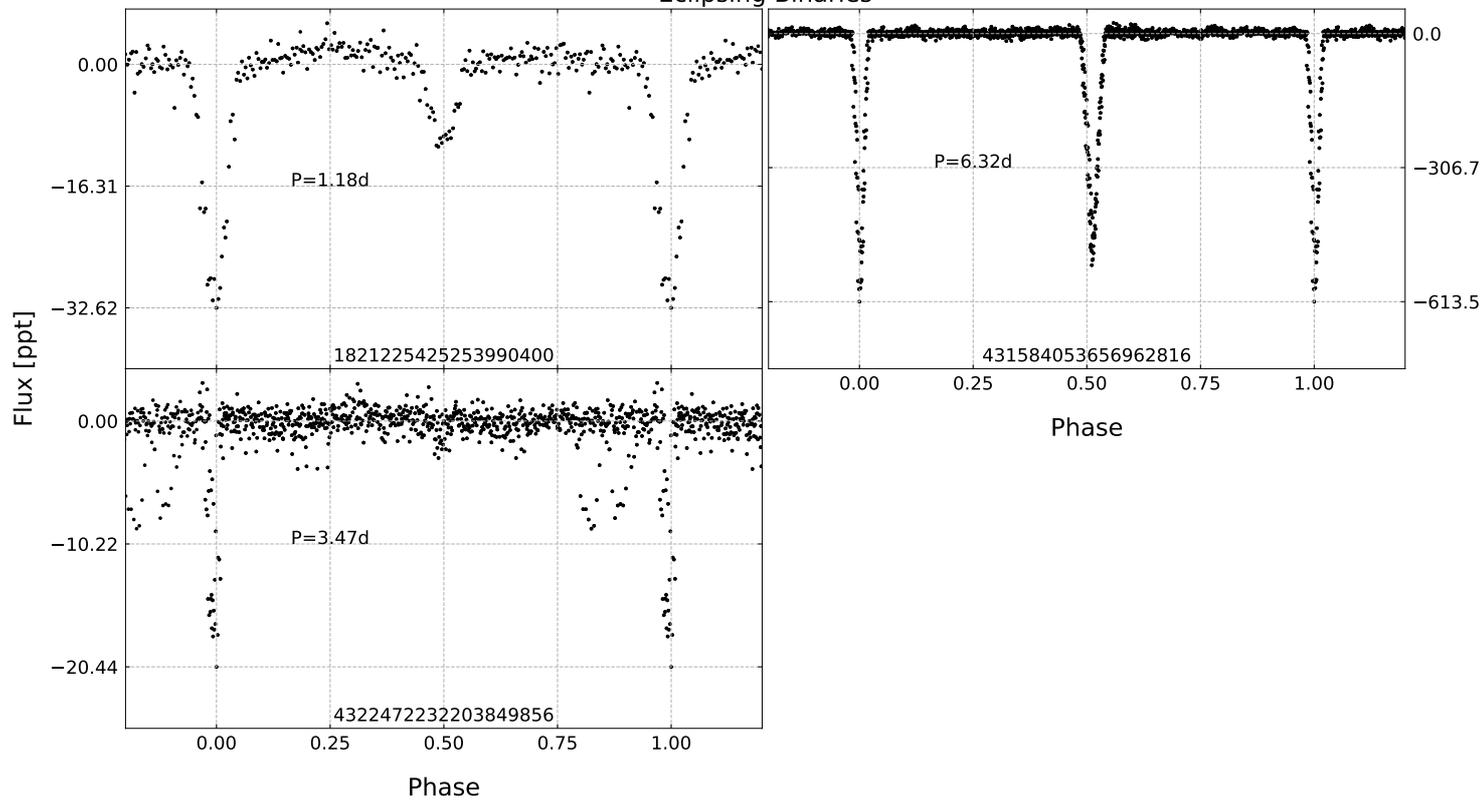

Phased lightcurves

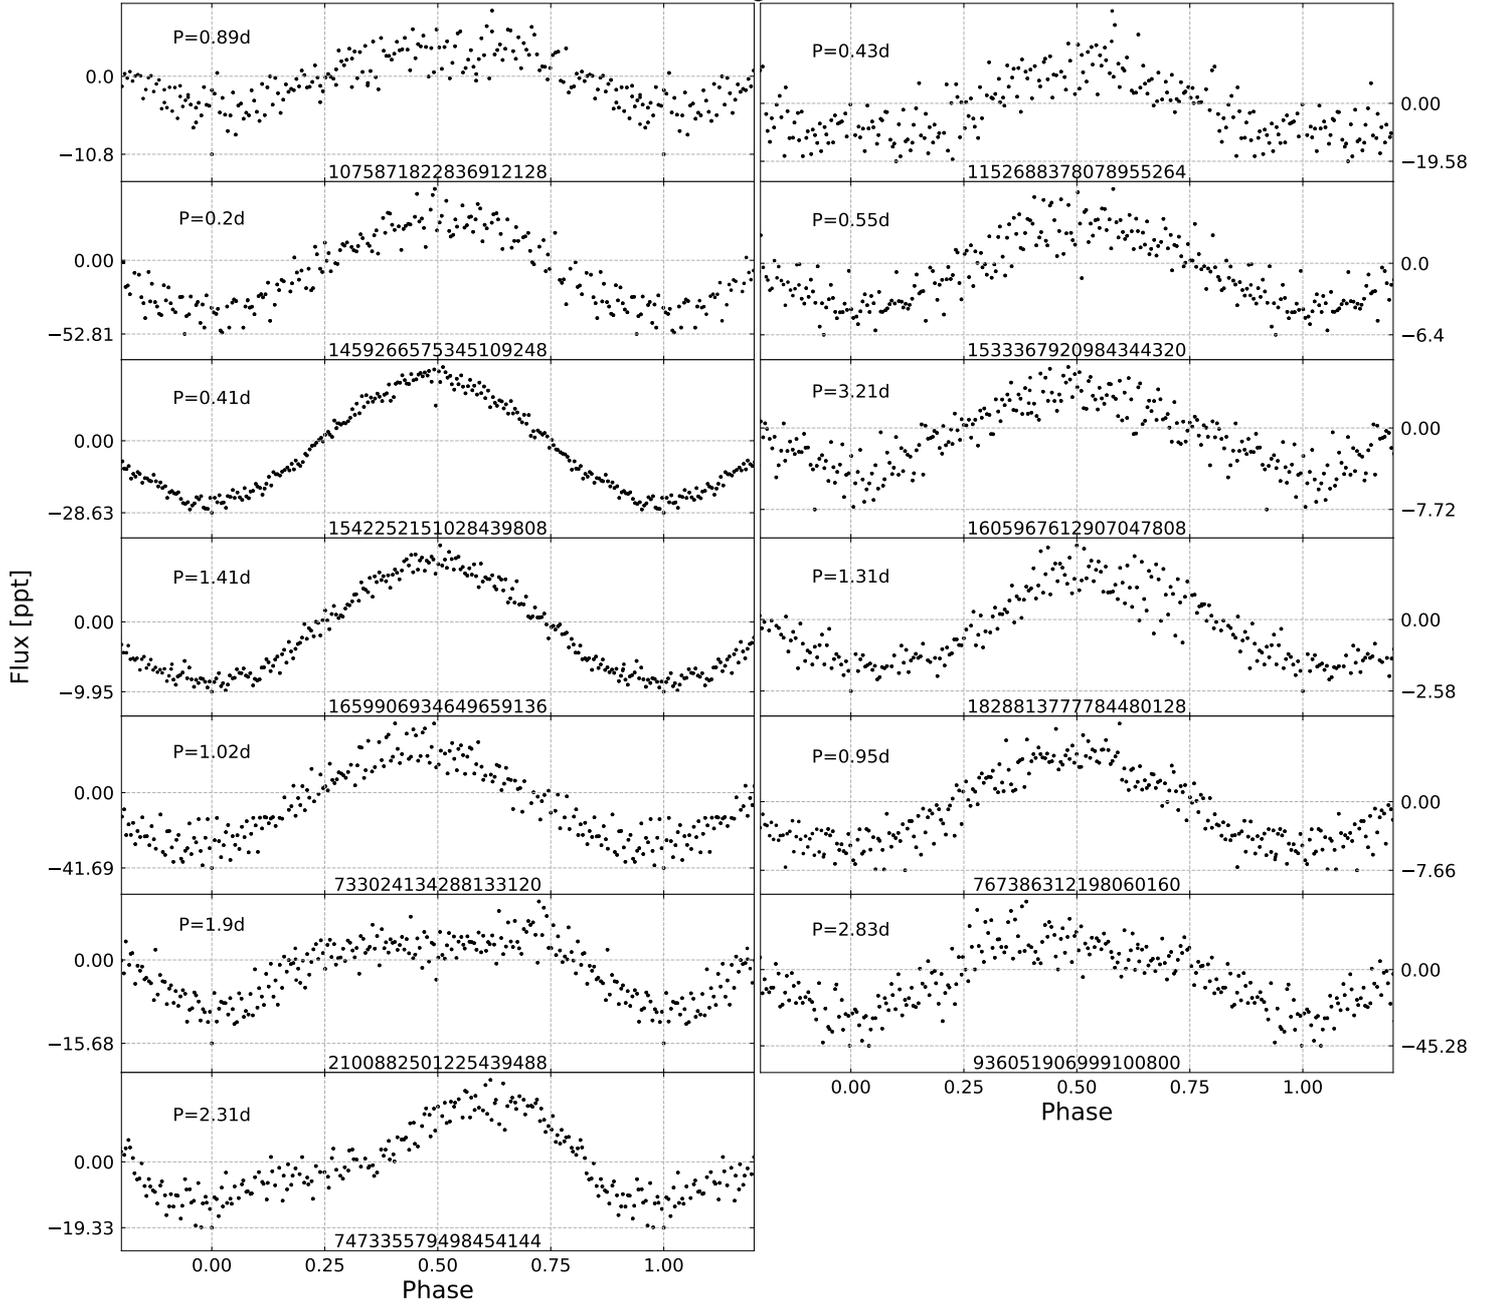

## Amplitude spectra

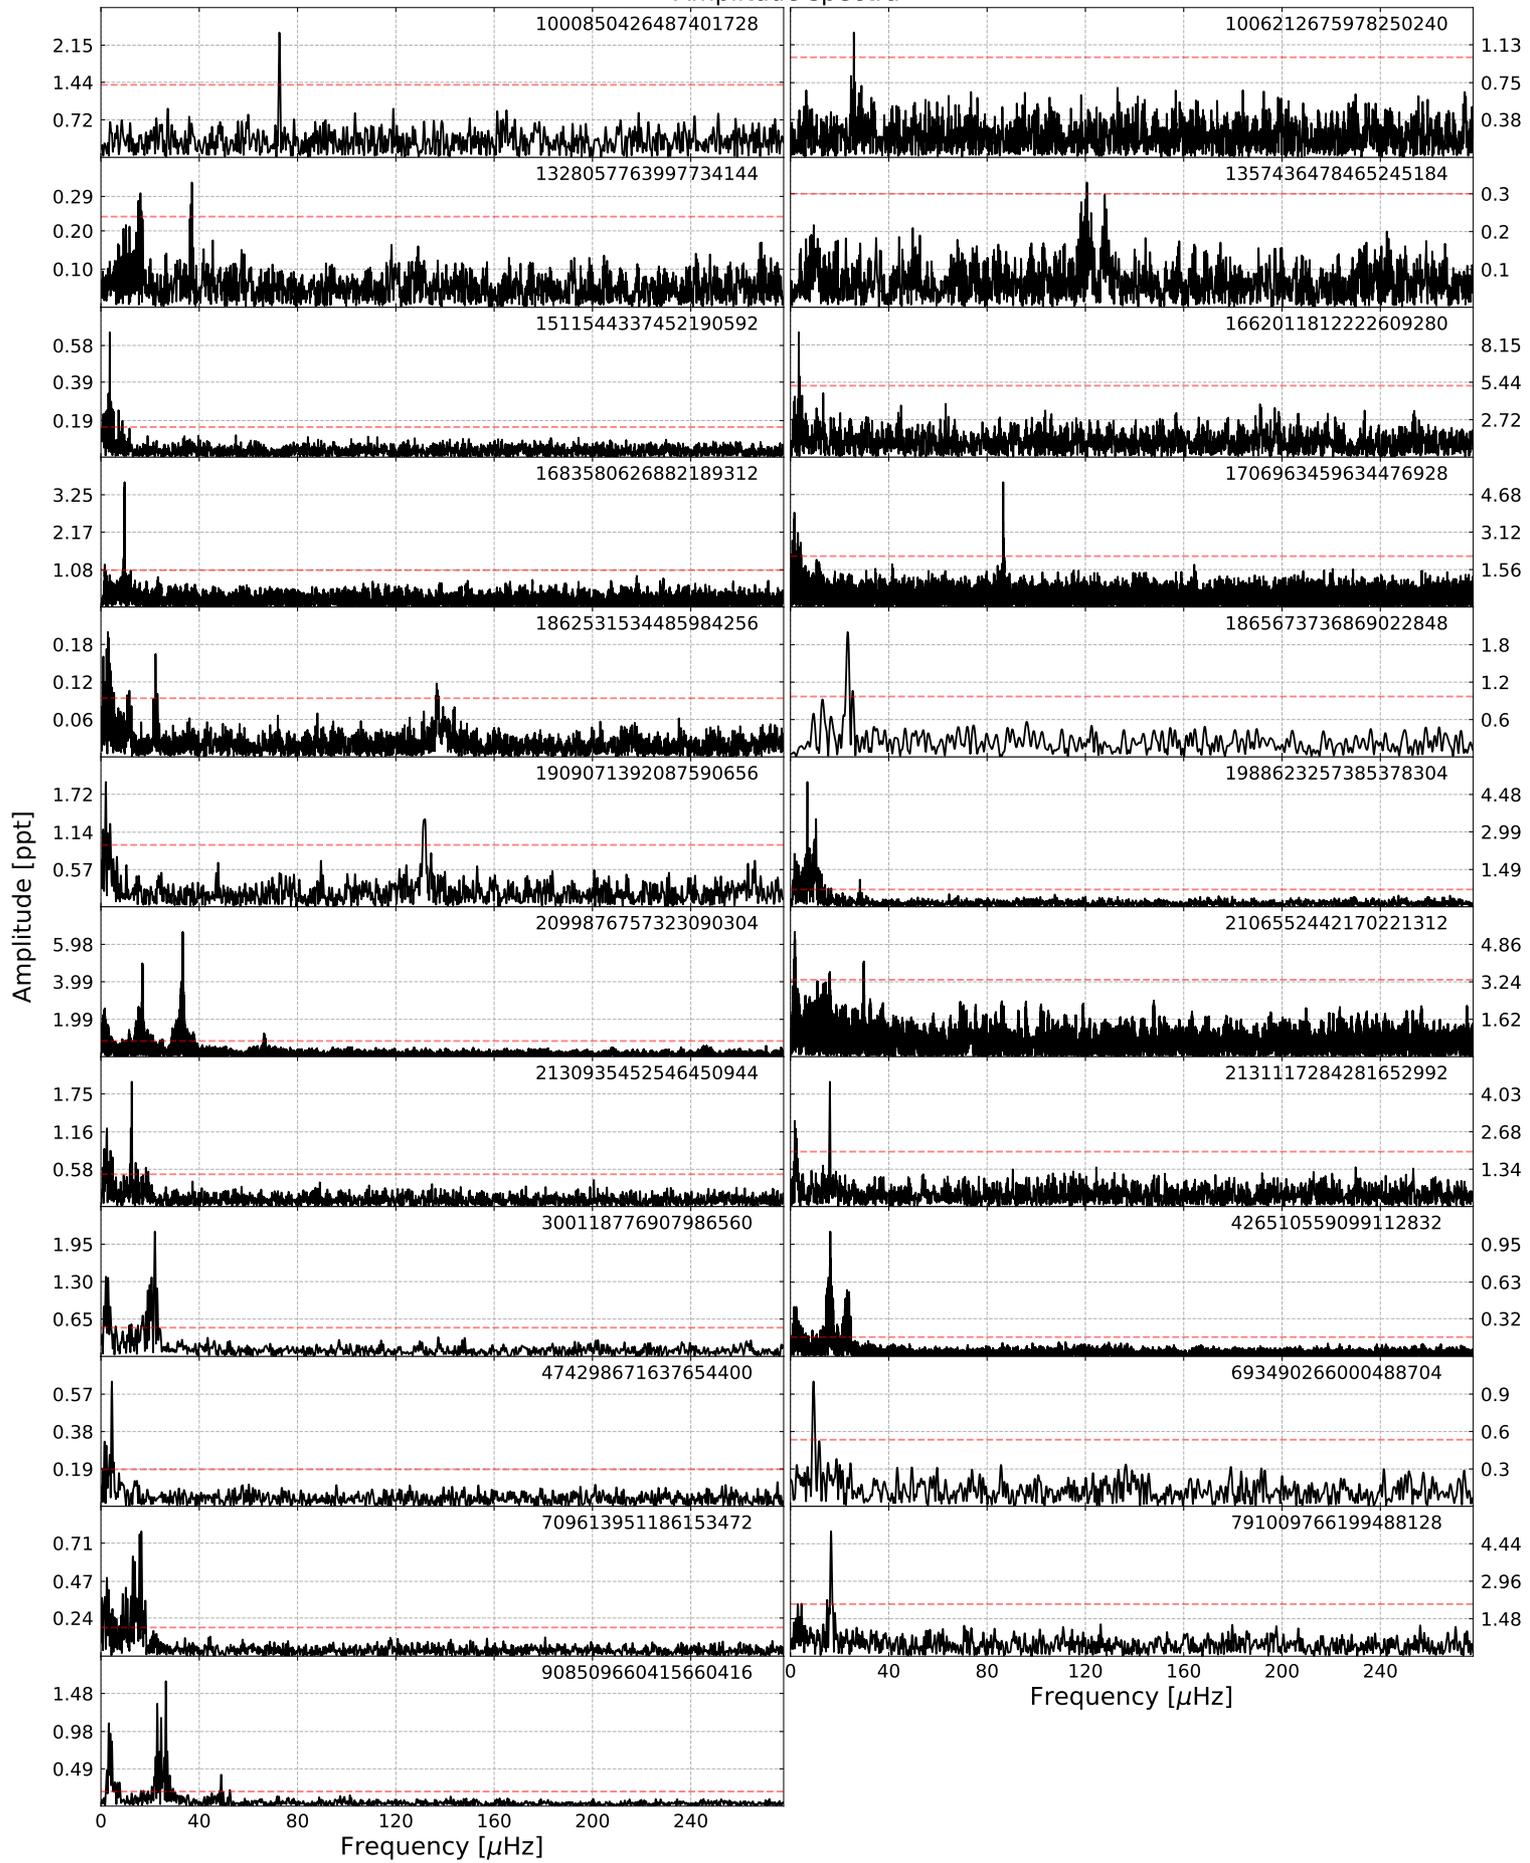

Supplement: Supplementary file 1 [file known_spec.pdf]
