# Supplementary material for: A search for variable subdwarf B stars in TESS Full Frame Images II. Variable objects in the northern ecliptic hemisphere
Source: arXiv:2105.01077 ancillary file (2021-05-03)

**Basic information of 228 spectroscopically unclassified variables.**  
**The table is followed by the amplitude spectra of these objects.**

| Gaia DR2            | TIC        | G<br>[mag] | Sector            | Remarks              |
|---------------------|------------|------------|-------------------|----------------------|
| 1082306439760979840 | 743148169  | 18.8118    | 20                | -                    |
| 1107705772542003200 | 705157619  | 18.0851    | 19,20,26          | object 18" away      |
| 1108642968765677696 | 743476657  | 18.7446    | 20,26             | -                    |
| 1112770367915047424 | 705166070  | 17.4131    | 19,20,26          | -                    |
| 1113516073020001152 | 705175423  | 18.3226    | 19,20,26          | object 18" away      |
| 124179878329719936  | 137965683  | 14.3788    | 18                | -                    |
| 1299121920781686912 | 345646956  | 16.4504    | 25                | -                    |
| 1316367176548009088 | 1200490403 | 18.9338    | 24,25             | -                    |
| 1328058588631578752 | 57188215   | 15.3725    | 24,25             | very crowded field   |
| 1360404507027046144 | 334900478  | 16.2607    | 25,26             | very crowded field   |
| 1360404644463437184 | 1270830822 | 16.3613    | 25,26             | very crowded field   |
| 1360404713182626176 | 1270831583 | 15.8418    | 25,26             | very crowded field   |
| 1360405366019600128 | 1270835502 | 16.6286    | 25,26             | very crowded field   |
| 1360405572181496576 | 334899867  | 16.2057    | 25,26             | very crowded field   |
| 1360405606536917888 | 1270837848 | 16.3565    | 25,26             | very crowded field   |
| 1360405640896788608 | 334899799  | 16.4277    | 25,26             | very crowded field   |
| 1360408252238042752 | 1270841916 | 16.4757    | 25,26             | very crowded field   |
| 1360408561479212416 | 1270843280 | 16.5303    | 25,26             | very crowded field   |
| 1360408694620012416 | 334899806  | 16.153     | 25,26             | very crowded field   |
| 1360408698917922304 | 1270843742 | 15.9875    | 25,26             | very crowded field   |
| 1360408870716557568 | 334899706  | 16.16      | 25,26             | very crowded field   |
| 1360409386112764800 | 334855274  | 15.6251    | 25,26             | crowded field        |
| 1366750338385213184 | 188823525  | 15.4073    | 24,25,26          | -                    |
| 1408611838431462272 | 1270929100 | 18.8069    | 24                | very crowded field   |
| 141362010961304960  | 433413657  | 11.9762    | 18                | -                    |
| 1454780812716838400 | 1000656229 | 18.0202    | 23                | very crowded field   |
| 1454781259395191168 | 1000658319 | 17.2302    | 23                | very crowded field   |
| 1454784557930979072 | 1000667332 | 17.7921    | 23                | very crowded field   |
| 1454785275190719616 | 416607024  | 16.7159    | 23                | very crowded field   |
| 1454875301999567104 | 199498039  | 16.3178    | 23                | crowded field        |
| 1454875400782264192 | 1000678734 | 17.0253    | 23                | crowded field        |
| 1638908908259733888 | 1401027720 | 18.1455    | 14-19,21-22,24-26 | -                    |
| 1641988266667804416 | 199550188  | 15.5435    | 14-26             | 2 objects within 30" |
| 1651395688155045888 | 1401049068 | 16.1897    | 14-25             | -                    |
| 1661867677415309440 | 1001372446 | 18.9922    | 15,16             | -                    |
| 1674177667865952000 | 1001488696 | 18.5485    | 14,15,21,22       | object 43" away      |
| 1792346408750425728 | 2001228745 | 18.4740    | 15                | -                    |
| 1800636593282297856 | 298659379  | 16.2993    | 15                | -                    |
| 1810293977574625536 | 1941781336 | 17.4479    | 14                | crowded field        |
| 1815926298906033280 | 1942976796 | 16.5239    | 14                | object 19" away      |
| 1816177434235193216 | 1943061704 | 18.1458    | 14                | crowded field        |

|                     |            |         |       |                             |
|---------------------|------------|---------|-------|-----------------------------|
| 1816244500139424128 | 1943089437 | 18.1146 | 14    | crowded field               |
| 1816360464255460608 | 1943134495 | 17.3974 | 14    | 3 objects within 21"        |
| 1818494070870971904 | 1943792185 | 17.6344 | 14    | crowded field               |
| 1818722769293285888 | 1943865981 | 16.8523 | 14    | 2 objects within 21"        |
| 1820808405423071616 | 1842059775 | 17.6540 | 14    | very crowded field          |
| 1823649504799178624 | 1945335720 | 18.8533 | 14    | crowded field               |
| 1824783277431088512 | 392156280  | 15.9607 | 14    | very crowded field          |
| 1838024657256337280 | 1950832039 | 17.2225 | 15    | -                           |
| 1838679897466100352 | 1950905363 | 18.7538 | 15    | object 15" away             |
| 1840251511899151360 | 1951113422 | 17.3028 | 15    | 4 bright objects within 32" |
| 1840546765129724928 | 2001826392 | 16.8209 | 15    | -                           |
| 1844179929505618560 | 1951817789 | 17.9994 | 14,15 | crowded field               |
| 1846296802929256832 | 1952256069 | 17.6588 | 15    | 4 bright objects within 21" |
| 1851085549721748608 | 298652703  | 13.2791 | 15    | -                           |
| 1855647423465451520 | 1953033063 | 18.4158 | 14,15 | 2 bright objects within 21" |
| 1858179465616300672 | 1954064238 | 17.3066 | 14,15 | 3 bright objects within 21" |
| 1866242253097646592 | 1957839690 | 17.4903 | 15    | crowded field               |
| 1866281247095593600 | 1957854845 | 17.3425 | 15    | -                           |
| 1866461223403421952 | 1957921006 | 17.4861 | 15    | 4 objects within 21"        |
| 1898657883100188544 | 162180176  | 13.2856 | 15,16 | -                           |
| 1901046606471675904 | 100594664  | 13.3995 | 16    | 3 objects within 21"        |
| 1905951734001545856 | 2003638995 | 17.3323 | 16    | -                           |
| 1906486401592241024 | 2003680569 | 17.8357 | 15,16 | 2 objects within 21"        |
| 1917952899121466368 | 374138533  | 12.1785 | 16    | -                           |
| 193414231450777216  | 700897252  | 18.8694 | 19    | 4 objects within 32"        |
| 1935580888012230784 | 2041819494 | 18.8264 | 16    | object 8" away              |
| 1935962732084366592 | 154818961  | 14.2472 | 16,17 | -                           |
| 1939760166070592000 | 431631481  | 14.2350 | 17    | 2 objects within 21"        |
| 1943858286426802304 | 2042696692 | 16.4713 | 17,24 | crowded field               |
| 1945729968750061440 | 287598689  | 15.4310 | 15    | 2 objects within 21"        |
| 1946614560216587008 | 287860863  | 14.6261 | 15,16 | 3 objects within 21"        |
| 1947213759696113920 | 426980323  | 15.8443 | 15    | 2 objects within 21"        |
| 1948774379006908288 | 2004376628 | 18.0547 | 15,16 | 2 bright objects within 21" |
| 1949931924236412032 | 256780950  | 13.0555 | 15,16 | 3 objects within 21"        |
| 1953745271081325440 | 304964655  | 16.2334 | 16    | 3 objects within 21"        |
| 1956067989393212032 | 2005522236 | 17.6484 | 15,16 | crowded field               |
| 1957707666169667456 | 2005732051 | 18.8639 | 16    | 2 objects within 21"        |
| 1964567764034901120 | 418537177  | 15.9802 | 15,16 | crowded field               |
| 196726961201325568  | 440388793  | 12.9139 | 19    | -                           |
| 1972683877836057600 | 419714501  | 15.6412 | 15,16 | crowded field               |
| 1979429038083843328 | 2011754031 | 15.245  | 16    | crowded field               |
| 1983619032071794944 | 2012994650 | 18.4314 | 16    | 2 objects within 21"        |
| 1985567439691237376 | 252527122  | 16.0067 | 16,17 | crowded field               |
| 1985860695759886592 | 2043377471 | 17.5606 | 16,17 | crowded field               |
| 1986759649594678528 | 2013148272 | 18.9822 | 16    | 3 objects within 21"        |
| 1987039337863810816 | 2013196679 | 18.9375 | 16    | 4 objects within 21"        |

|                     |            |         |          |                                                                 |
|---------------------|------------|---------|----------|-----------------------------------------------------------------|
| 1987437812052513536 | 467529837  | 14.0629 | 16       | crowded field                                                   |
| 1992525217991908480 | 2044370599 | 14.4129 | 17,24    | 3 bright objects within 21"                                     |
| 1995466995705902592 | 2045012618 | 18.5430 | 16,17    | crowded field                                                   |
| 2001188476275895936 | 2014205738 | 18.9117 | 16,17    | crowded field                                                   |
| 2001383841438971136 | 2014292802 | 16.9613 | 16,17    | crowded field                                                   |
| 2001659926247735040 | 431145331  | 15.2748 | 16,17    | crowded field                                                   |
| 2032857194333300352 | 1867908327 | 17.0787 | 14       | very crowded field                                              |
| 2034597824311822848 | 57507655   | 14.3920 | 14       | very crowded field                                              |
| 2037262318906365312 | 1712166670 | 18.3812 | 14       | 4 bright objects within 21"                                     |
| 2037415700780608128 | 1712233248 | 15.653  | 14       | 3 bright objects within 21"                                     |
| 2037478025041657472 | 1712262553 | 17.1789 | 14       | 4 bright objects within 21"                                     |
| 2039324521683150080 | 403248740  | 13.9044 | 14       | crowded field                                                   |
| 2039459241912570880 | 1712945849 | 18.3612 | 14       | 5 objects within 21"                                            |
| 2040412174897885184 | 1713259626 | 18.1840 | 26       | 3 objects within 21"                                            |
| 2041930329878249984 | 20439718   | 15.3262 | 14,26    | 3 bright objects within 21"                                     |
| 2042199985105098496 | 28858086   | 14.7076 | 14,26    | crowded field                                                   |
| 2045244429726676608 | 1873354652 | 18.1498 | 14       | very crowded field                                              |
| 2077210973653321600 | 1880746153 | 18.8867 | 14,15    | 4 objects within 21"                                            |
| 2079330419753334144 | 1881387607 | 17.8125 | 14,15    | crowded field                                                   |
| 2080459759936046464 | 271547244  | 14.7670 | 14,15    | 2 bright objects within 21"                                     |
| 2080623857747831424 | 271659828  | 16.2105 | 14,15    | 5 objects within 21"                                            |
| 2080657500231447808 | 1881707922 | 18.3566 | 14,15    | KIC 10676210 22" away                                           |
| 2083565811572191360 | 193863012  | 16.5079 | 14,15    | crowded field                                                   |
| 2086397839981036032 | 1881890367 | 18.0990 | 14,15    | 5 objects within 21"                                            |
| 2087153483644941568 | 1882061796 | 16.8658 | 14,15    | crowded field                                                   |
| 2088226705776949888 | 1973057768 | 18.2006 | 14,16    | 3 bright objects within 21"                                     |
| 2088337756446382464 | 1973089618 | 17.8223 | 14,15,16 | 4 bright objects within 21"                                     |
| 2090760637700298112 | 1714998110 | 17.8327 | 14,26    | 2 objects within 21"                                            |
| 2091025070244210944 | 68265412   | 13.3638 | 26       | -                                                               |
| 2092946501174006528 | 1715312730 | 16.9082 | 14       | -                                                               |
| 2093324767535333888 | 237183273  | 14.5774 | 14,26    | 4 objects within 21"                                            |
| 2098226081131178880 | 336132473  | 13.1182 | 14,26    | Gaia DR2 2098226081131180288<br>11" away                        |
| 2098353109083521664 | 336263242  | 16.2593 | 14,26    | 2 objects within 32"                                            |
| 2099796218097223552 | 1715938427 | 17.5197 | 14       | object 16" away                                                 |
| 2100070954267036672 | 1715980555 | 17.7709 | 14       | 2 objects within 21"                                            |
| 2101160913887221888 | 1882248573 | 17.5637 | 14       | 5 objects within 21"                                            |
| 2103059117632458368 | 1716331834 | 18.7842 | 14       | 4 bright objects within 21"                                     |
| 2105585421693855744 | 158424730  | 17.2767 | 14       | CV ( <a href="#">Scaringi et al. 2013</a> )                     |
| 2111853428244955264 | 1550574605 | 16.1897 | 14,26    | 4 objects within 32"                                            |
| 2113739326907805696 | 1550678705 | 18.6456 | 25,26    | 3 objects within 21"                                            |
| 2115076131184395520 | 7804997    | 15.2431 | 14,26    | -                                                               |
| 2126207243307096192 | 1882483337 | 18.9311 | 15       | 3 bright objects within 21"                                     |
| 2127444125171341312 | 1882631458 | 16.7283 | 15       | KIC 9278505<br>( <a href="#">Reinhold et al. 2013</a> ) 9" away |
| 2127850772675551232 | 1882665005 | 17.0644 | 15       | object 19" away                                                 |
| 2128309711401769344 | 1882735968 | 18.9031 | 14,15    | 5 objects within 21"                                            |

|                     |            |         |                      |                             |
|---------------------|------------|---------|----------------------|-----------------------------|
| 2128316411551020160 | 1882737149 | 18.8877 | 14,15                | object 19" away             |
| 2129409566628271232 | 290035516  | 16.0203 | 14,15                | 2 objects within 21"        |
| 2129683074442759040 | 1882937348 | 16.7850 | 14,15                | 4 objects within 21"        |
| 213308657404832768  | 664834496  | 16.7240 | 19                   | 4 objects within 21"        |
| 2137421299839603328 | 27998017   | 14.9175 | 14,15,16             | -                           |
| 2137489984956949632 | 1883388858 | 17.7692 | 15,16                | 2 objects within 32"        |
| 2138054511159522432 | 1883465325 | 18.4798 | 14,16                | 3 objects within 21"        |
| 2138263800623825024 | 1883489297 | 17.5481 | 14,15,16             | crowded field               |
| 2141313261762604032 | 377197425  | 16.6398 | 14-16,19-20,22-23,26 | object 9" away              |
| 2159159709869671168 | 233120549  | 15.6365 | 14-19,21-26          | 3 objects within 21"        |
| 2161688071217417728 | 233064123  | 9.5177  | 15-16,18,21,24-25    | 3 objects within 4"         |
| 2166781146535333888 | 366849840  | 15.8878 | 15,16                | bright object 15" away      |
| 2171574772400722048 | 2016922661 | 16.3448 | 15,16                | crowded field               |
| 2218305807587114624 | 411576480  | 15.9979 | 16,18,24             | 2 objects within 32"        |
| 2219210568217622912 | 412363512  | 16.8612 | 16,18,24             | 3 objects within 21"        |
| 2231467614602883456 | 367090060  | 15.2675 | 17,18,19,24,25       | -                           |
| 2233797475444252288 | 1980585525 | 18.9924 | 14                   | 3 objects within 21"        |
| 2233846442371207168 | 233266154  | 15.9960 | 14,16                | 4 objects within 21"        |
| 2234034351481581568 | 1980600166 | 18.7514 | 14-16                | 2 bright objects within 21" |
| 2234114173452564096 | 1883770385 | 17.7281 | 14-16                | 4 objects within 21"        |
| 2234624553006762624 | 1980637218 | 16.8607 | 14-17                | 4 objects within 21"        |
| 2236210461089760000 | 1980673962 | 16.5330 | 14-17                | 3 bright objects within 32" |
| 2237409719037840384 | 256622207  | 16.9954 | 14-17,24             | 4 bright objects within 21" |
| 2237551517380084736 | 1883954695 | 16.2242 | 14-17,21,24          | 4 objects within 21"        |
| 2238098803590426368 | 256384536  | 14.1767 | 14-18,21,24          | crowded field               |
| 2239900383454607232 | 1884092103 | 17.3801 | 14-26                | 2 bright objects within 32" |
| 2244819843293381376 | 236888904  | 15.6813 | 15-18,21,24-25       | 2 objects within 21"        |
| 2254710740659370496 | 229962636  | 14.3874 | 14-15,17-26          | -                           |
| 2260984927665960704 | 1884416085 | 18.8718 | 14-26                | object 16" away             |
| 2261060214149311872 | 259170065  | 16.0001 | 14-26                | -                           |
| 2271591989352943488 | 1981426661 | 18.6153 | 16-19,24-25          | 3 objects within 21"        |
| 2287403962995179264 | 2051677111 | 16.9138 | 18,19,25,26          | -                           |
| 265031711598697728  | 321831910  | 14.9658 | 19                   | -                           |
| 270172340774799488  | 306211983  | 15.7534 | 19                   | -                           |
| 2863196315306344832 | 419547639  | 15.3922 | 17                   | -                           |
| 316139833851242240  | 61337611   | 11.0826 | 17                   | -                           |
| 318144999462982912  | 620805781  | 18.3142 | 17                   | object 11" away             |
| 336682765508713728  | 381730939  | 12.1039 | 18                   | object 9" away              |
| 341218594570556032  | 621422778  | 17.2222 | 18                   | 5 objects within 21"        |
| 343903292727125504  | 28690361   | 16.0099 | 17,18                | -                           |
| 3444031646422921344 | 309113421  | 16.2609 | 19                   | 5 objects within 21"        |
| 347293568112654720  | 189598026  | 16.5705 | 17                   | object 16" away             |
| 355680848969498368  | 301100606  | 15.3465 | 18                   | 2 objects within 21"        |
| 359675851453158656  | 622557069  | 18.3911 | 18                   | 4 objects within 21"        |
| 359799649588750464  | 250453464  | 15.1130 | 18                   | crowded field               |
| 375930000563894784  | 191663789  | 11.5158 | 17                   | -                           |



|                     |            |         |             |                             |
|---------------------|------------|---------|-------------|-----------------------------|
| 390486812962336256  | 601419369  | 18.7112 | 17          | 3 objects within 32"        |
| 3938022150401267072 | 953956379  | 17.6395 | 23          | very crowded field          |
| 398116839542946944  | 196946103  | 14.4348 | 17,18       | object 16" away             |
| 408964281963069696  | 403400154  | 16.1295 | 18          | 5 objects within 21"        |
| 412544287524575744  | 623638028  | 17.7800 | 18          | 5 objects within 21"        |
| 417769377238431744  | 240716329  | 16.2234 | 17,18       | 5 objects within 21"        |
| 420571242106123776  | 603886634  | 15.3484 | 17,24       | crowded field               |
| 424739456329229824  | 604803910  | 18.5798 | 17,18       | crowded field               |
| 431525298501730816  | 359039906  | 16.7213 | 17,18,24    | 2 bright objects within 21" |
| 4497574170517871616 | 1681600851 | 17.4273 | 26          | 4 objects within 21"        |
| 4498708419837302400 | 1681874891 | 18.4054 | 26          | 4 objects within 21"        |
| 4500054462584536576 | 1505807101 | 16.9482 | 26          | object 4" away              |
| 4502102302993010688 | 1682046125 | 17.2885 | 26          | 3 objects within 21"        |
| 4510156191310953984 | 462811965  | 16.0340 | 26          | 5 objects within 21"        |
| 4511999243375875584 | 1683377714 | 18.0770 | 26          | crowded field               |
| 4519583124826317568 | 1811394469 | 17.0293 | 14          | crowded field               |
| 4523127954613606912 | 1683842358 | 17.9957 | 26          | 5 objects within 21"        |
| 4524788625192532864 | 1684271267 | 18.9618 | 26          | 4 objects within 21"        |
| 4527057879749609984 | 1684833800 | 18.8265 | 26          | crowded field               |
| 4528076581574683008 | 1685008842 | 17.6761 | 26          | 5 objects within 21"        |
| 4528846617674457472 | 342320091  | 14.5273 | 26          | 4 objects within 21"        |
| 4530859303765646336 | 1813173164 | 18.9596 | 26          | 5 objects within 21"        |
| 4535895994733729024 | 1814885171 | 18.9764 | 26          | crowded field               |
| 4537278012127640576 | 1686111363 | 17.9216 | 26          | bright object 20" away      |
| 453810165809216512  | 249953635  | 15.0975 | 18          | 4 objects within 21"        |
| 4545156047299735936 | 1308564438 | 18.3925 | 25          | -                           |
| 4548857999871987712 | 1506415981 | 18.1587 | 26          | object 8" away              |
| 4553345622222014720 | 1506923479 | 17.0906 | 25,26       | 4 objects within 21"        |
| 4577858379269509248 | 1507563495 | 17.5297 | 26          | 5 objects within 32"        |
| 4587673444692894848 | 1815401960 | 17.2154 | 26          | 3 objects within 21"        |
| 4589093944995879936 | 377682650  | 16.3499 | 26          | 5 objects within 21"        |
| 4589221793281682048 | 313898581  | 15.7822 | 26          | 3 objects within 21"        |
| 4607166377101142272 | 76039505   | 15.7868 | 26          | -                           |
| 479934630799062656  | 82969837   | 16.9913 | 19          | -                           |
| 533041484802576512  | 379086469  | 16.2229 | 18,24,25    | 3 bright objects within 21" |
| 550070931346054784  | 103511037  | 15.1911 | 19,25,26    | 3 objects within 21"        |
| 559799478948924800  | 289267299  | 15.6577 | 18,19,25    | object 18" away             |
| 562049900075843072  | 629777697  | 17.2863 | 18,19,26    | object 14" away             |
| 573943493448464384  | 461601415  | 16.2667 | 18,20,25,26 | 3 objects within 21"        |
| 796315837515758720  | 4839754    | 13.6219 | 21          | -                           |
| 897707263615279872  | 741428427  | 17.9573 | 20          | object 17" away             |
| 898706032489528064  | 423081986  | 15.3837 | 20          | object 5" away              |
| 940404431153925632  | 741916679  | 17.4930 | 20          | -                           |
| 945273721477246208  | 15924748   | 15.4795 | 20          | object 18" away             |
| 951138134245928704  | 197181683  | 16.5237 | 20          | object 12 away              |
| 951495028848519424  | 742278003  | 18.2046 | 20          | 2 objects within 21"        |

|                    |           |         |    |   |
|--------------------|-----------|---------|----|---|
| 994967386444824064 | 11595640  | 13.0729 | 20 | - |
| 995053663747140352 | 444902249 | 10.8428 | 20 | - |
| 995329916043197952 | 258620986 | 15.8380 | 20 | - |
| 999919342001035648 | 743017950 | 16.9607 | 20 | - |

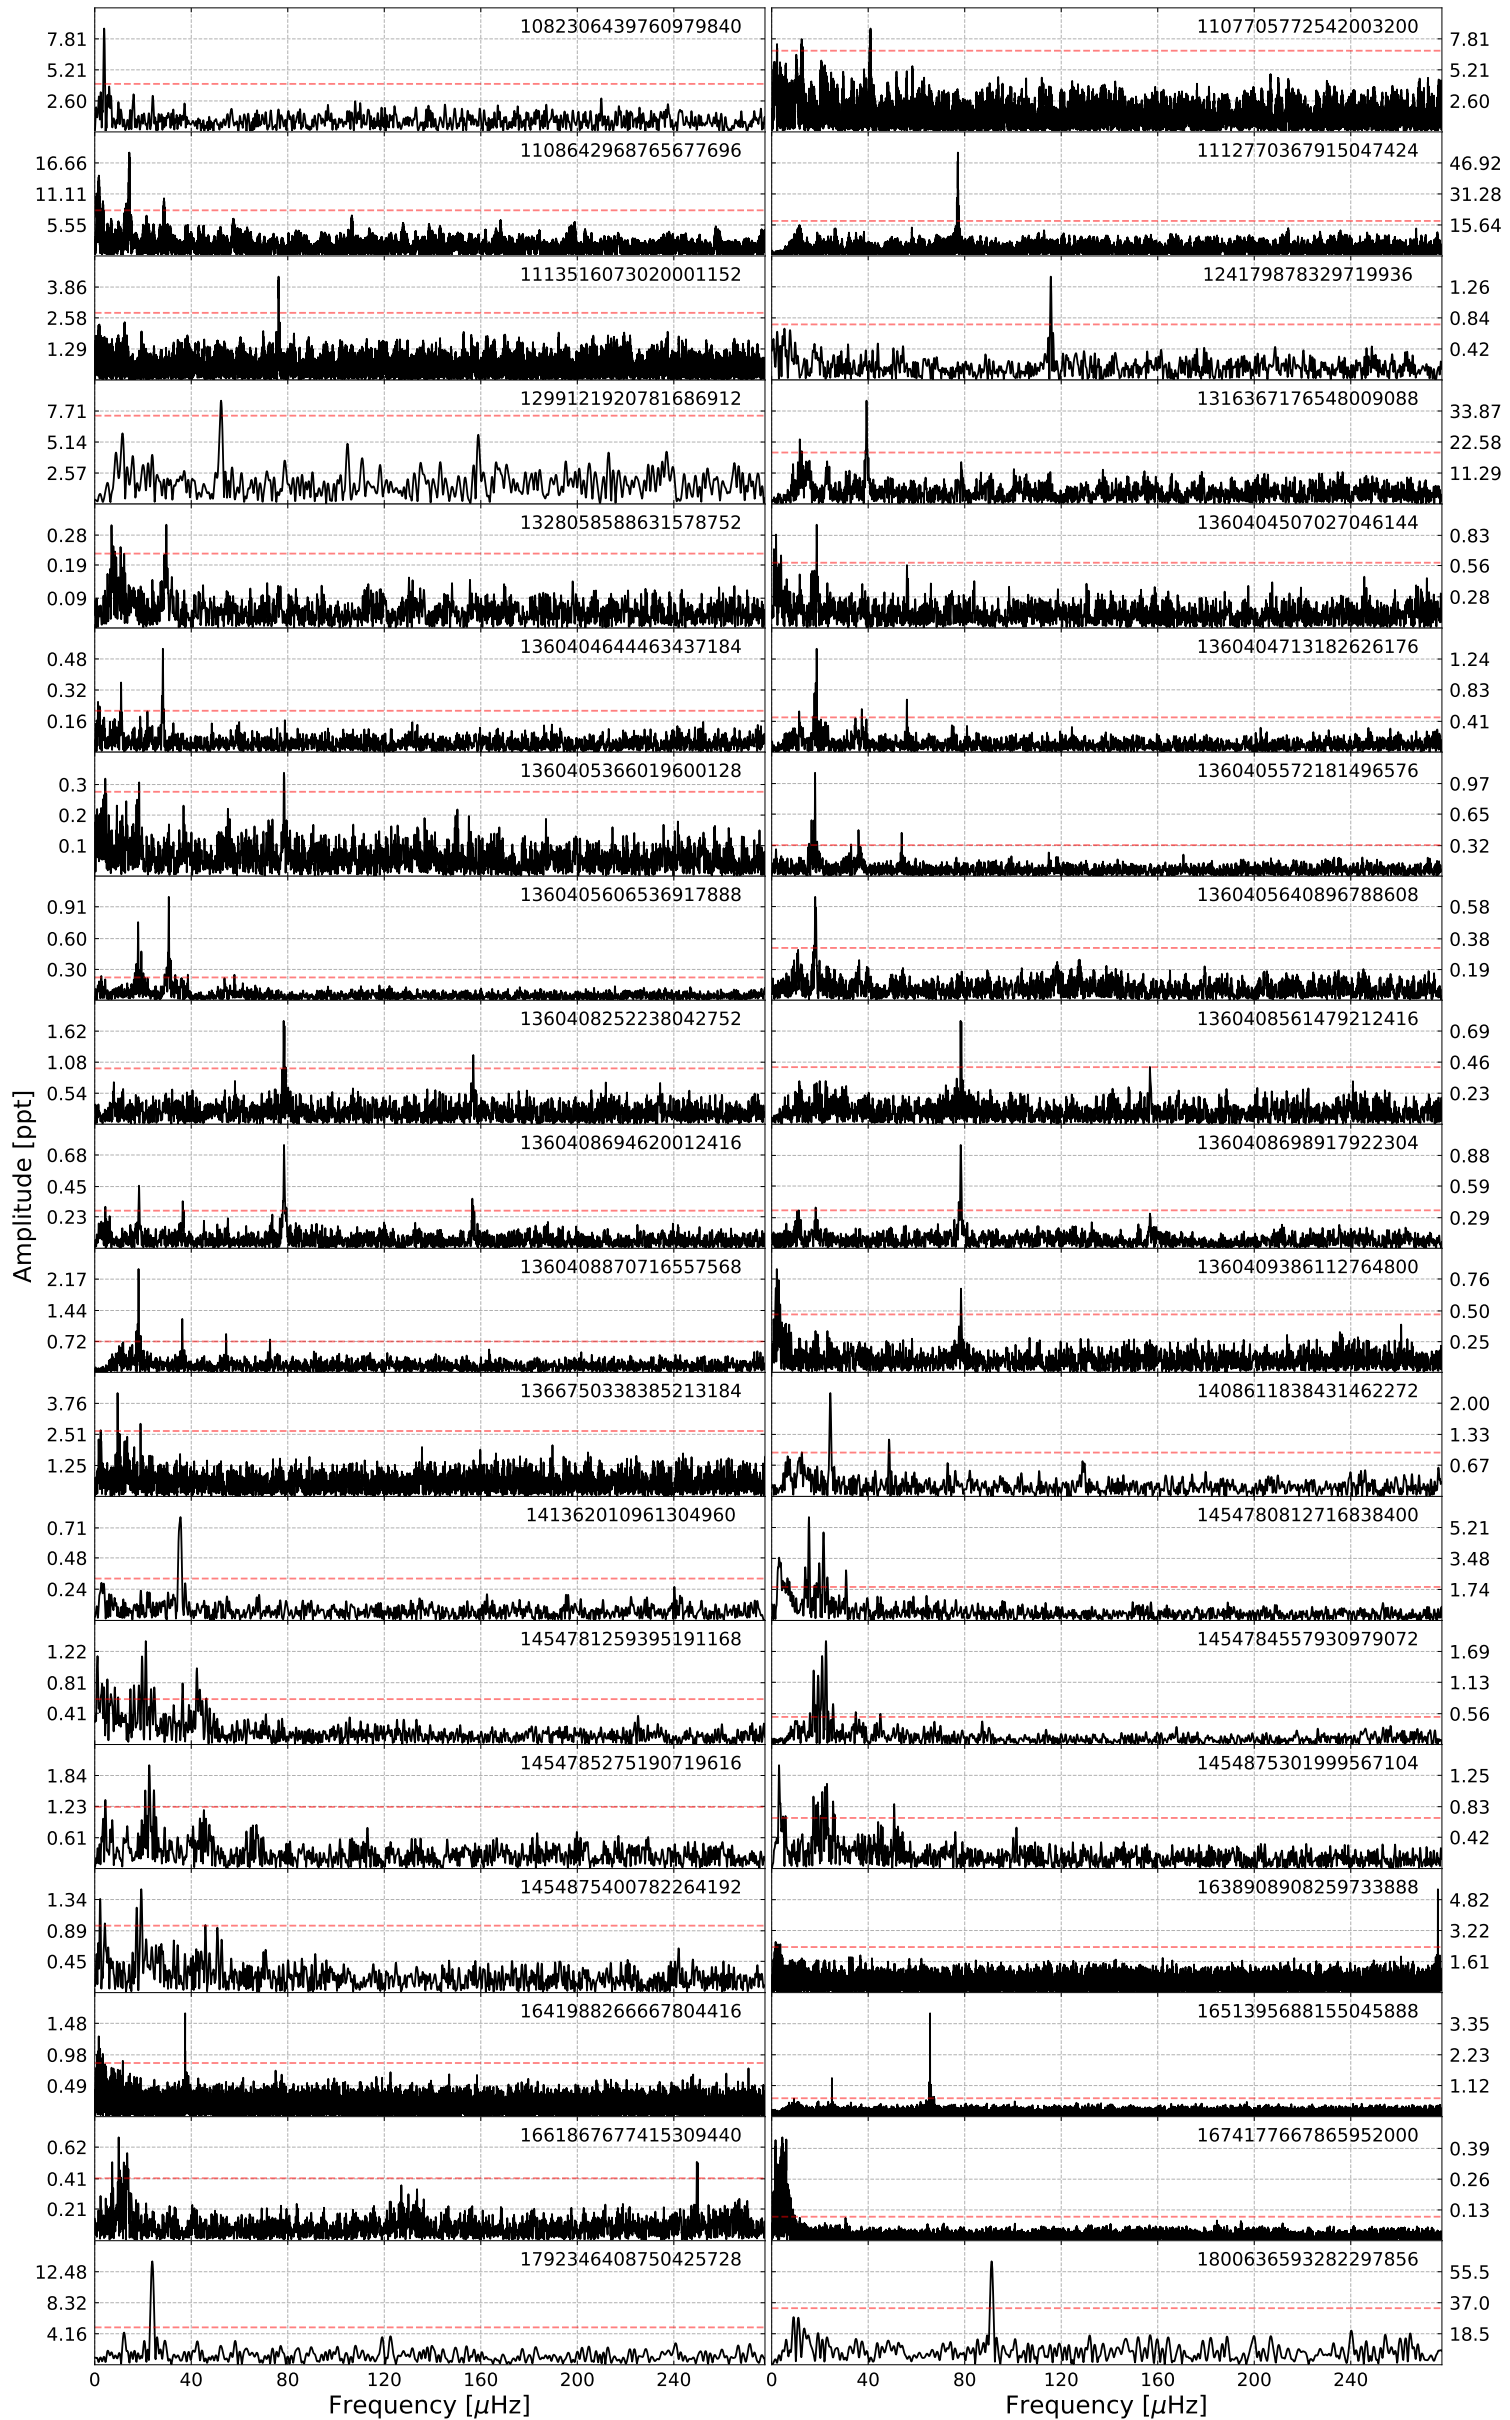

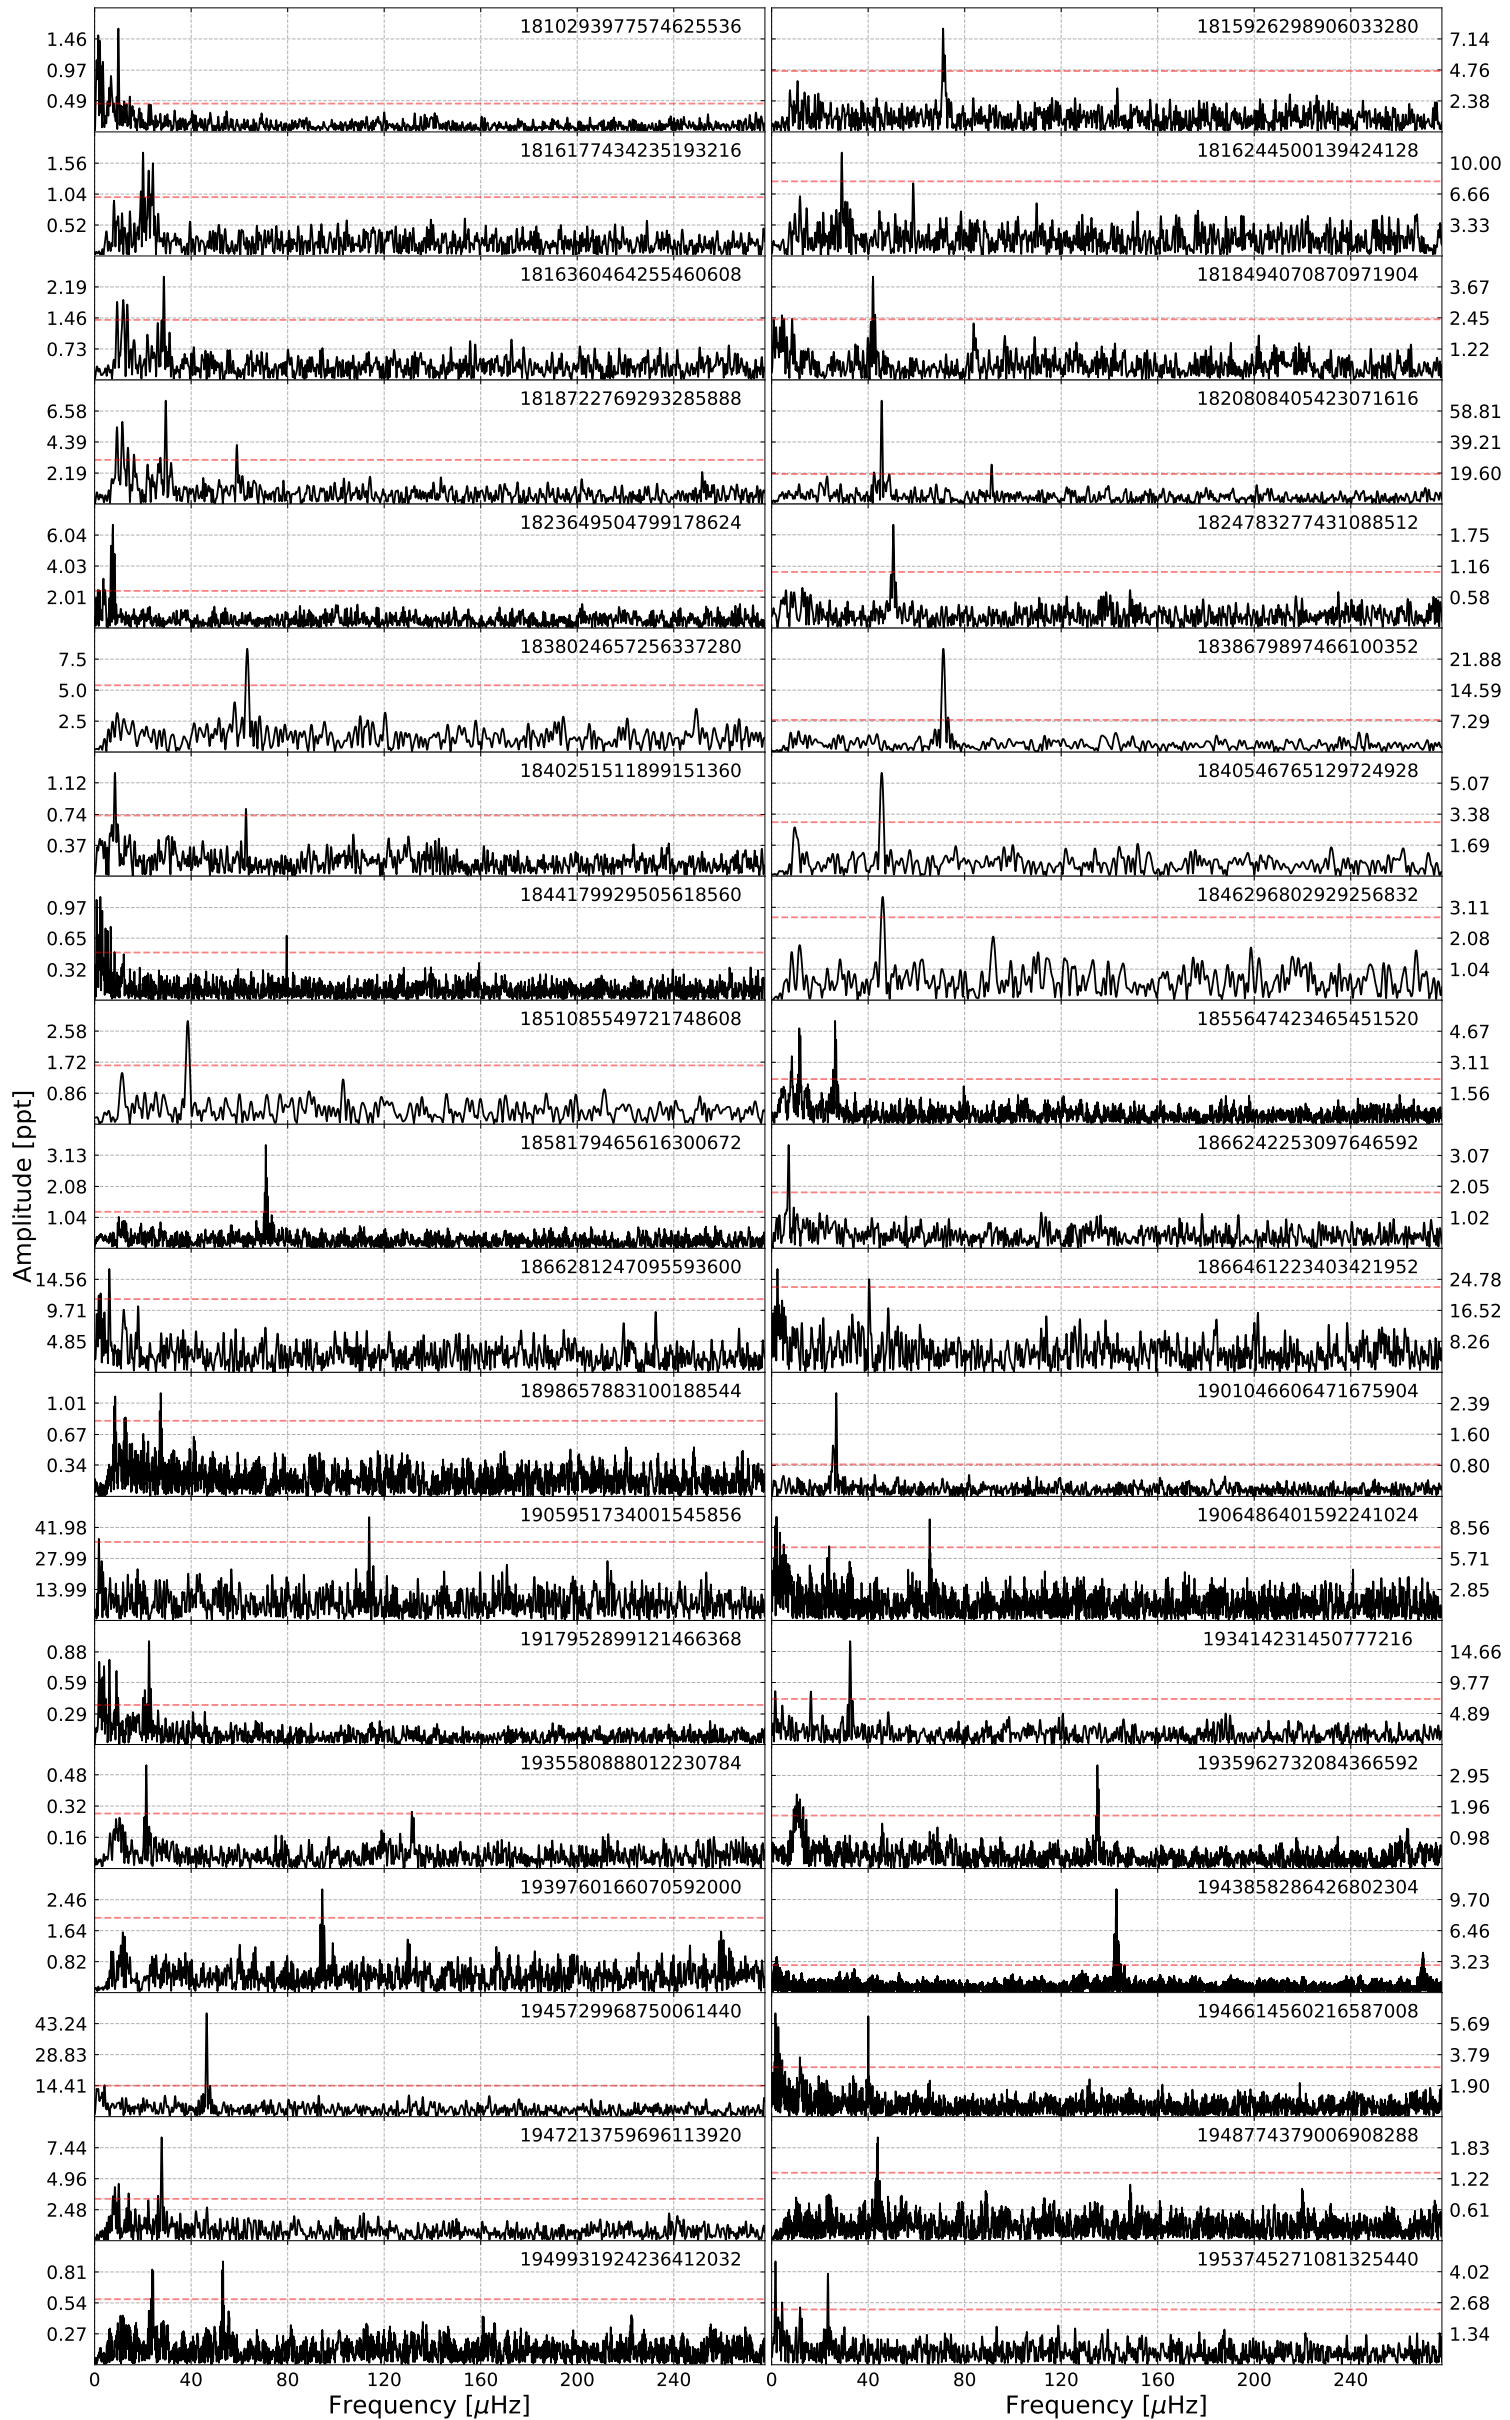

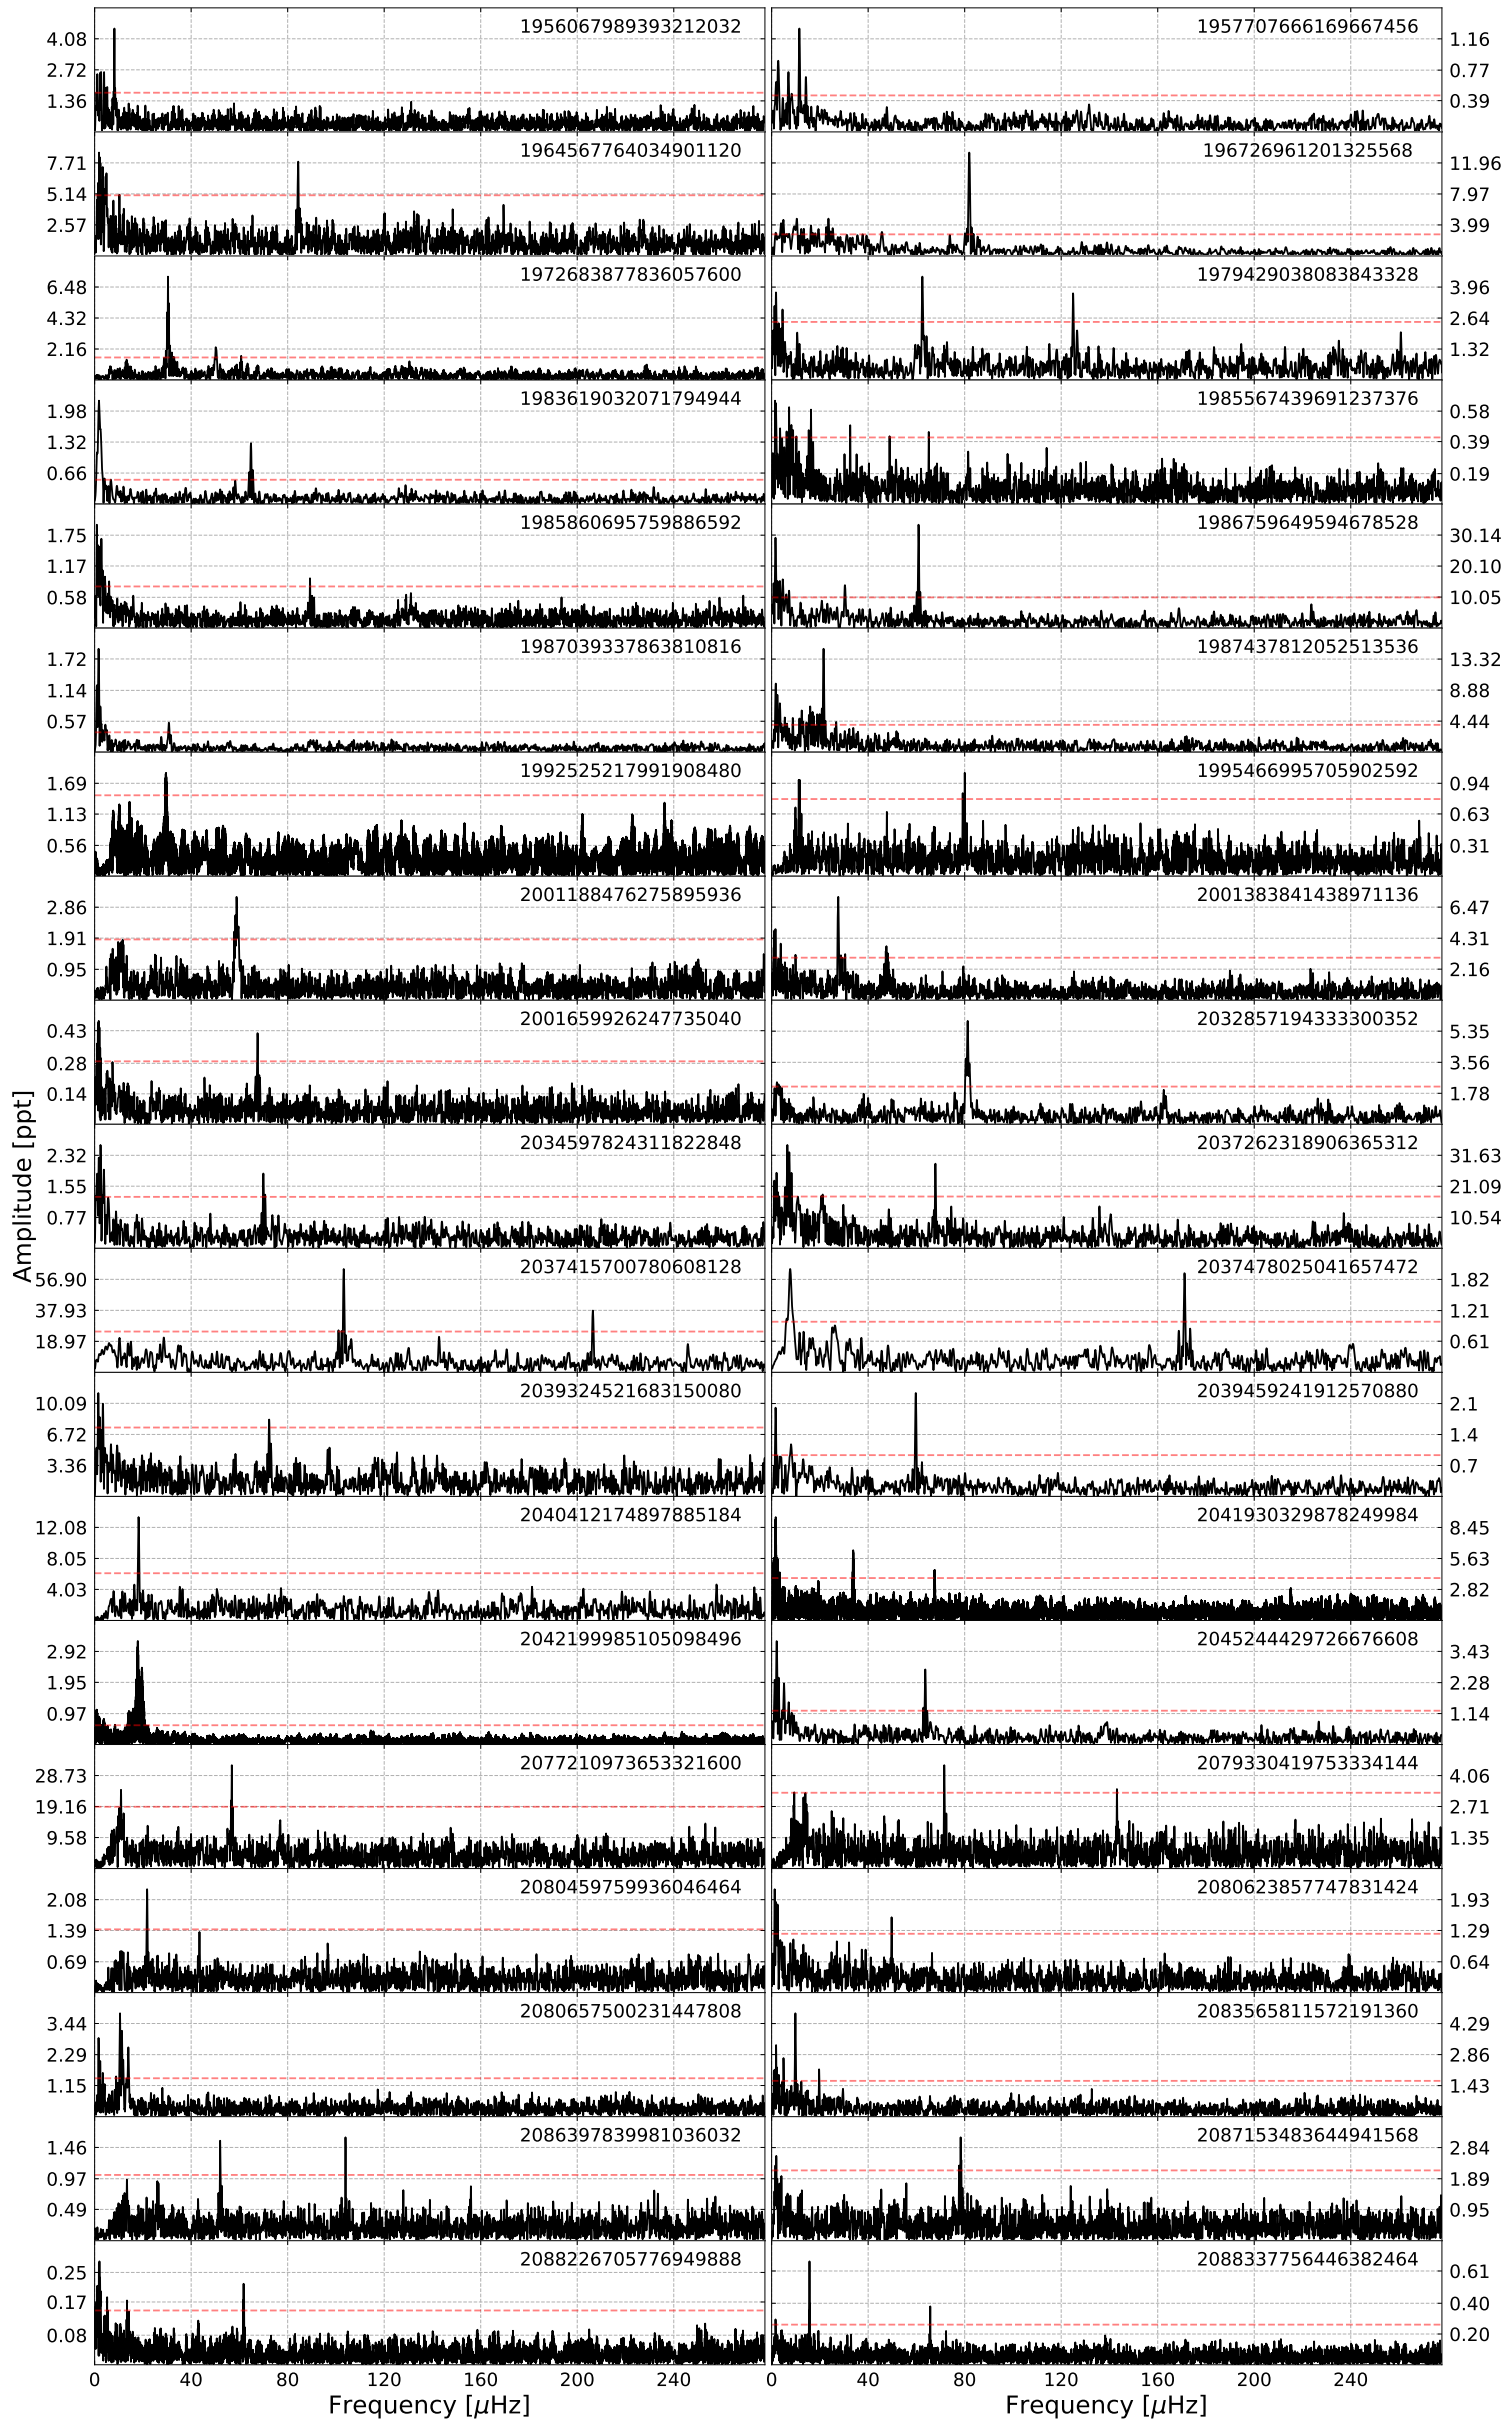



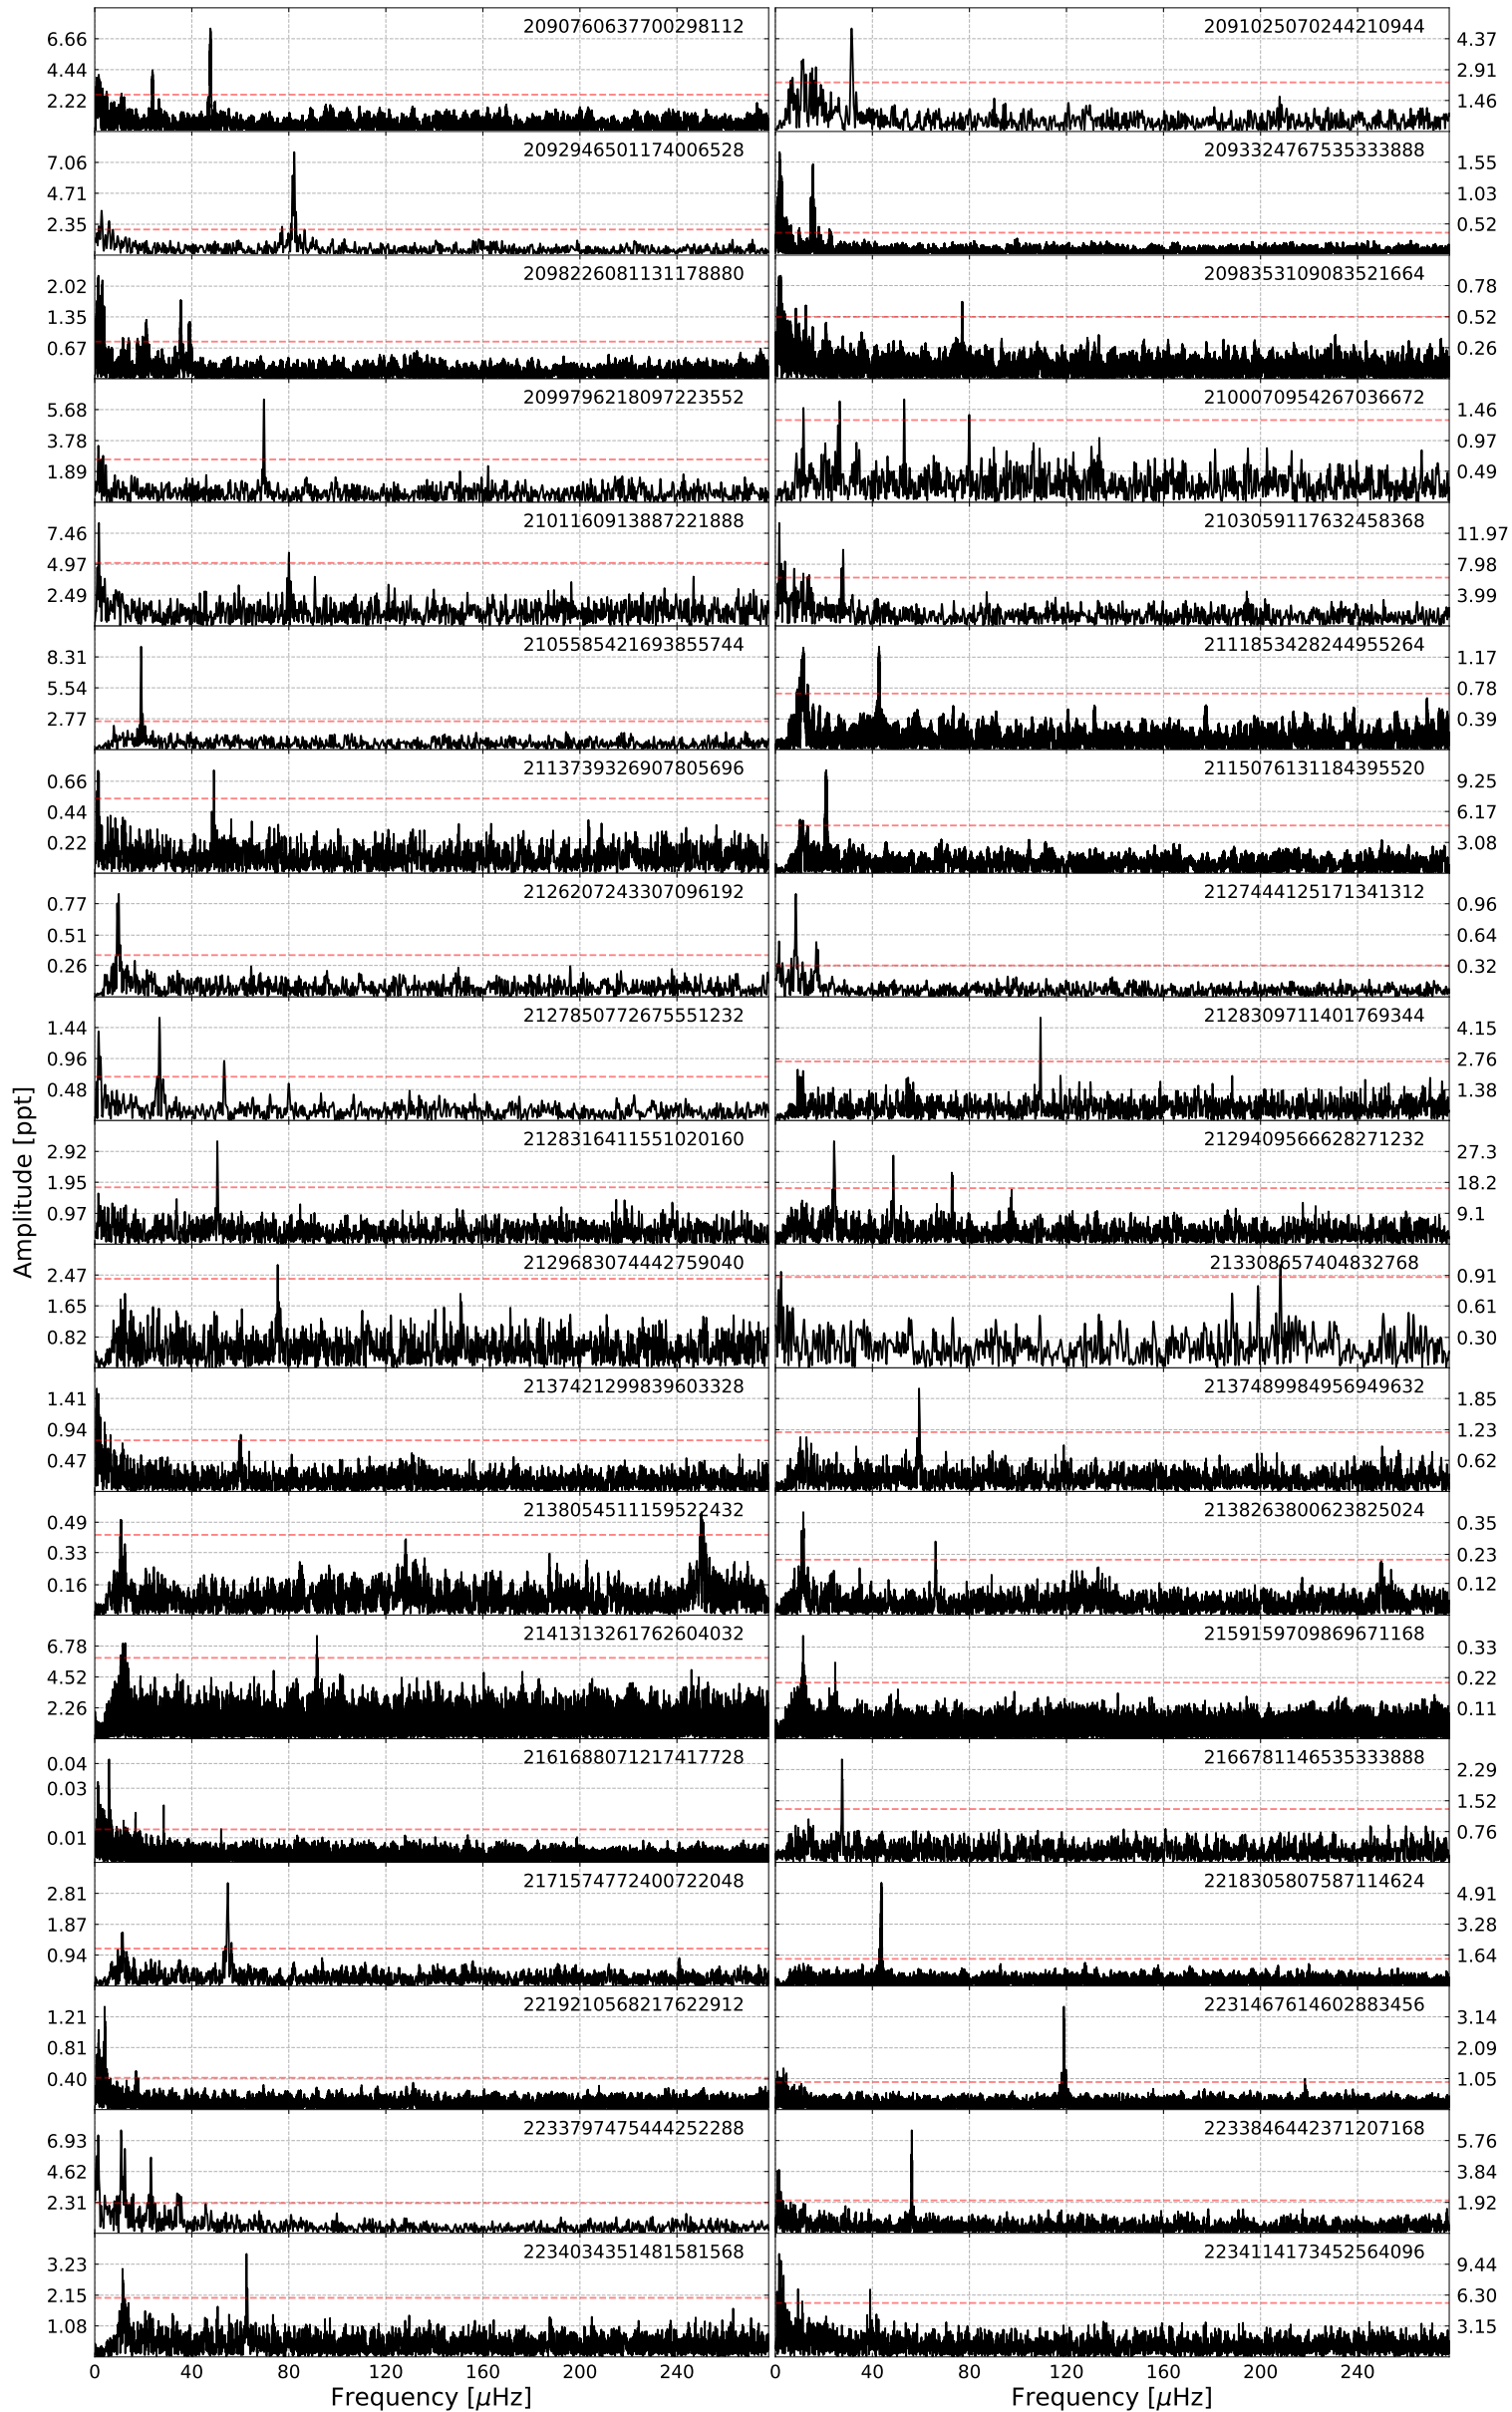

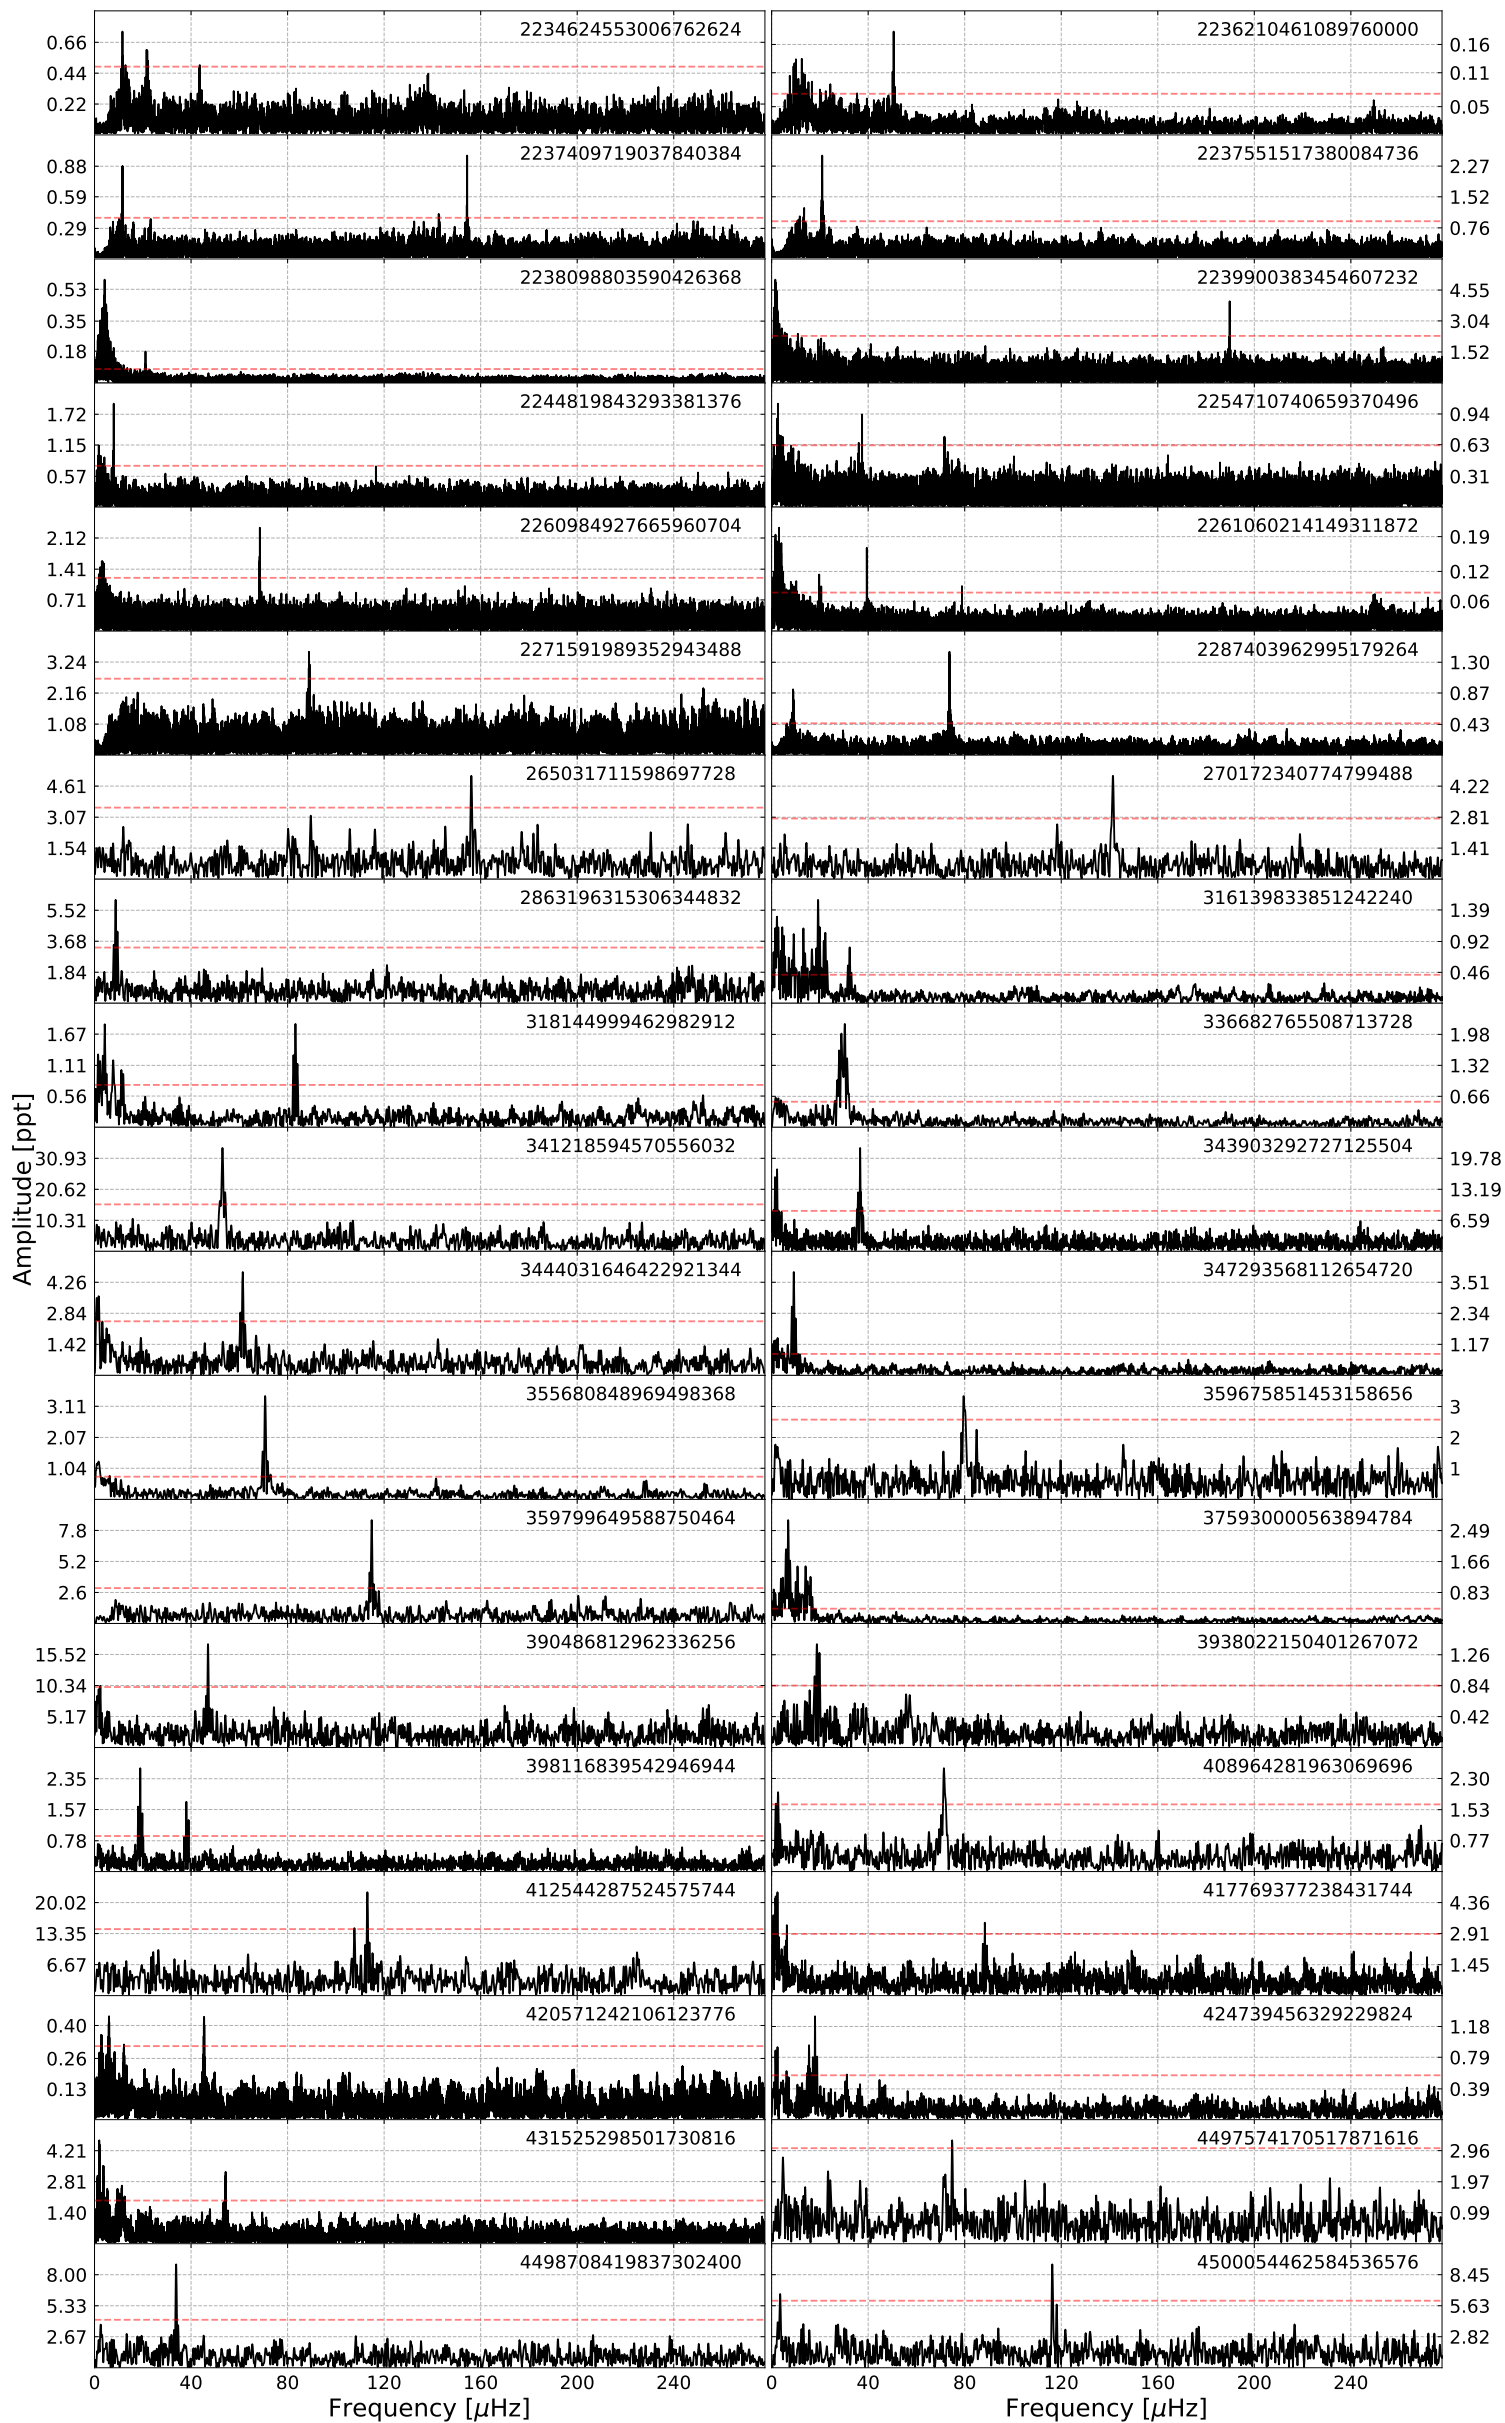

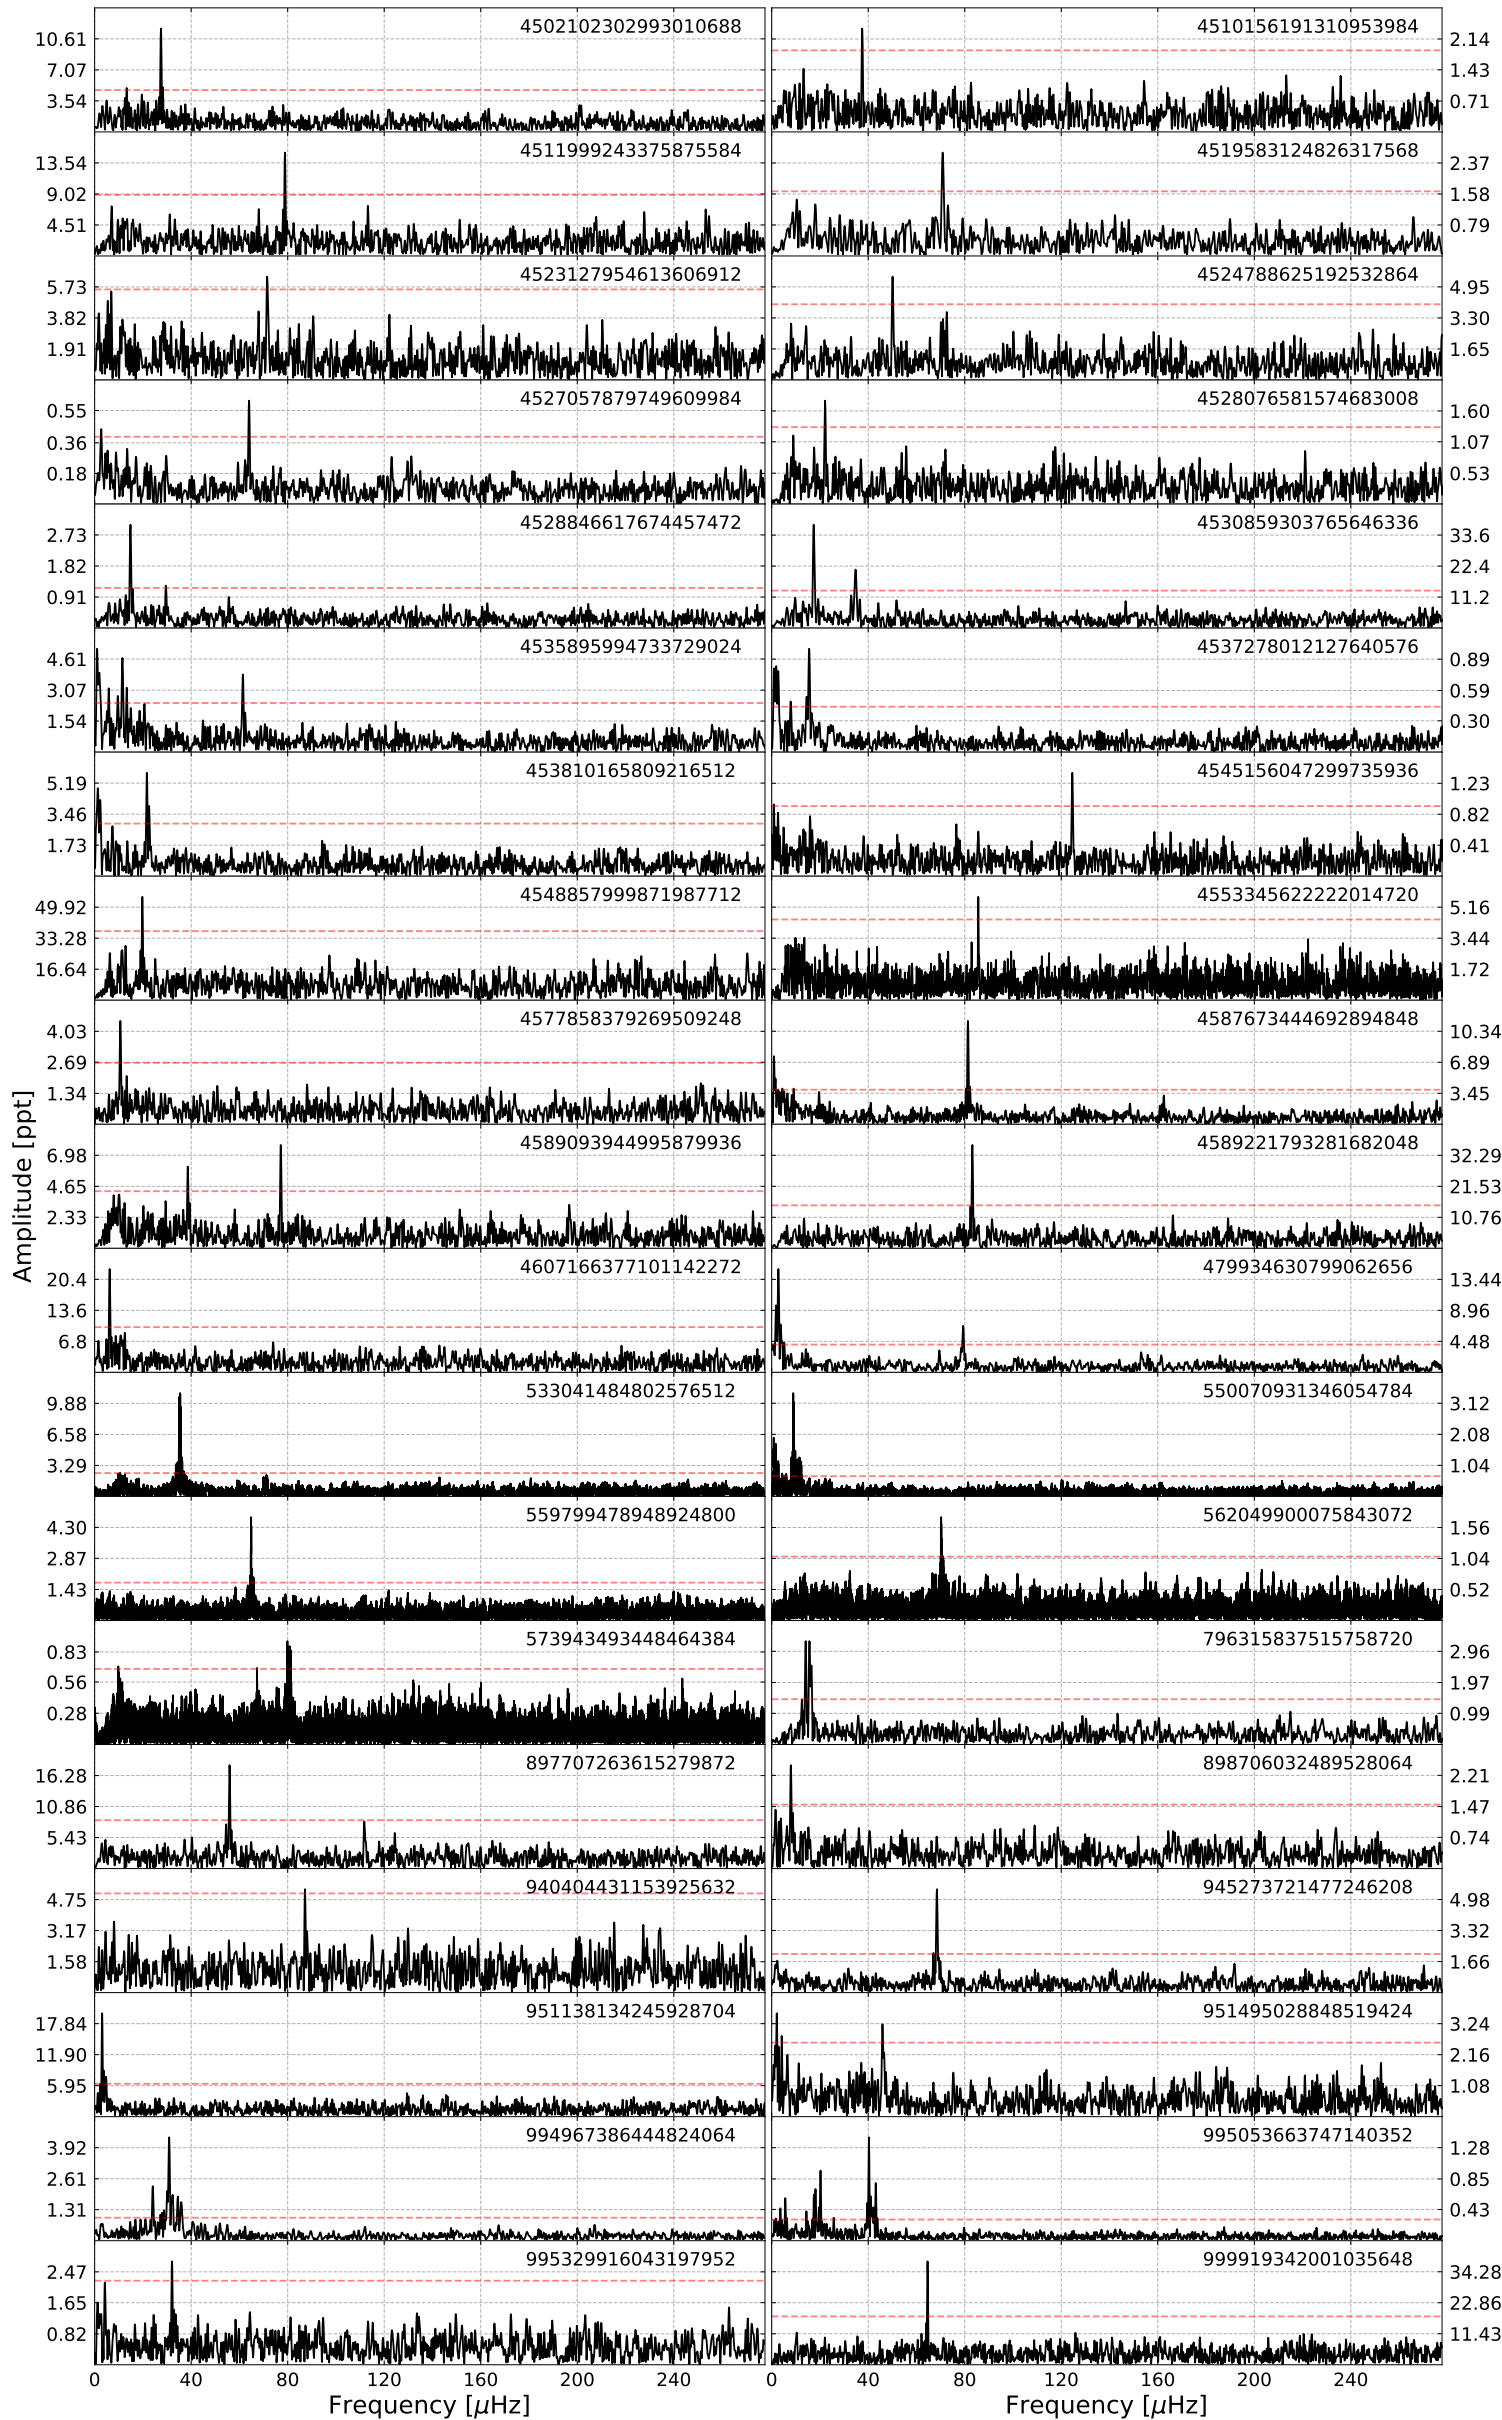

Supplement: Supplementary file 2 [file no_spec_fr.pdf]
