# Supplementary material for: A search for variable subdwarf B stars in TESS Full Frame Images II. Variable objects in the northern ecliptic hemisphere
Source: arXiv:2105.01077 ancillary file (2021-05-03)

**Basic information of 93 spectroscopically unclassified binaries without sharp eclipses.**  
**The table is followed by the phased time-series of these objects.**

| <i>Gaia</i> DR2                       | TIC        | G<br>[mag] | Sector            | Period<br>[days] | Remarks                     |
|---------------------------------------|------------|------------|-------------------|------------------|-----------------------------|
| <b>One symmetric maximum detected</b> |            |            |                   |                  |                             |
| 1000519267329142144                   | 444946935  | 15.9244    | 20                | 1.6725           | -                           |
| 1086341235118052096                   | 85158691   | 12.8544    | 20                | 0.3546           | -                           |
| 1099487030500185344                   | 743328948  | 16.8995    | 20                | 0.3297           | -                           |
| 1133795950814826240                   | 841399917  | 17.3147    | 14,20,26          | 1.5134           | 4 objects within 30"        |
| 1141625057721183616                   | 138400883  | 16.2436    | 19,20,26          | 0.0680           | object 23" away             |
| 1328061818442252032                   | 1270377531 | 17.5025    | 24,25             | 0.3913           | 3 bright objects within 2   |
| 1336799091888985600                   | 9569988    | 11.8732    | 25,26             | 2.7441           | -                           |
| 1344525738054881152                   | 116262175  | 14.4309    | 25,26             | 2.5163           | object 20" away             |
| 141494094091434880                    | 67658009   | 13.0436    | 18                | 0.8764           | -                           |
| 156955941997427456                    | 96951247   | 15.7180    | 19                | 0.1592           | -                           |
| 1708730890216076416                   | 159438888  | 14.4114    | 14-15,19-21,25-26 | 0.6370           | object 27" away             |
| 1816292363253864064                   | 1943106787 | 18.8576    | 14                | 0.8747           | crowded field               |
| 1816586516979325696                   | 1943243403 | 18.4249    | 14                | 0.2286           | crowded field               |
| 1817158988879945600                   | 219640470  | 14.1771    | 14                | 0.5359           | 4 objects within 21"        |
| 1831343410431617920                   | 406417817  | 14.7108    | 14                | 0.2010           | crowded field               |
| 1844828920542477568                   | 1951933220 | 16.5533    | 15                | 0.1909           | -                           |
| 1856240648652853760                   | 282366215  | 14.8348    | 14,15             | 0.6220           | crowded field               |
| 1893009515772824064                   | 2002921529 | 17.2982    | 15                | 0.2410           | -                           |
| 1896251498822626560                   | 18000205   | 14.0261    | 15                | 1.1013           | -                           |
| 1902886016408161280                   | 2040326958 | 17.6360    | 16                | 1.4690           | crowded field               |
| 1920489236226682496                   | 125489130  | 16.7815    | 16,17             | 0.1229           | object 18" away             |
| 1922534396571549184                   | 2040945100 | 18.1865    | 17                | 1.7462           | 3 objects within 21"        |
| 1973144057810900096                   | 427916222  | 16.2244    | 15,16             | 0.3723           | 3 objects within 21"        |
| 1997600078330802688                   | 345216287  | 16.4890    | 17,24             | 0.0935           | crowded field               |
| 2042814161128667136                   | 1713892529 | 18.9317    | 14                | 2.8649           | object 12" away             |
| 2046397439474347904                   | 1874192801 | 14.2467    | 14                | 0.5796           | crowded field               |
| 2050133678755873792                   | 1876676459 | 18.5065    | 14                | 0.7463           | crowded field               |
| 2050526964622031744                   | 1714628258 | 17.2228    | 14                | 0.5351           | -                           |
| 2068952271239193344                   | 193800883  | 15.1000    | 14,15             | 0.2926           | -                           |
| 2071550515996622592                   | 188973075  | 16.3566    | 15,16             | 1.0682           | 4 objects within 21"        |
| 2072903984764773248                   | 1879342714 | 17.8580    | 14                | 0.1761           | crowded field               |
| 2080900114347408384                   | 416641307  | 14.5962    | 14,15             | 0.3011           | 3 objects within 21"        |
| 2086292772201176320                   | 1881864796 | 17.2562    | 14,15             | 1.9530           | 3 objects within 21"        |
| 2088590094368104448                   | 1973148204 | 18.1677    | 14,15,16          | 0.7242           | 3 bright objects within 21" |
| 2089872678980572032                   | 1714844032 | 17.8843    | 14,26             | 5.6149           | 5 bright objects within 21" |
| 2091796510791468288                   | 68673218   | 13.7080    | 14,26             | 0.3164           | bright object 16" away      |
| 2101329963798339968                   | 1716151993 | 18.6796    | 14                | 0.3907           | KIC 5439660 21" away        |
| 2125305094015307520                   | 21018674   | 13.4058    | 14,15,18,21,25,26 | 1.5079           | -                           |
| 2126639381440599552                   | 1882566921 | 17.7115    | 15                | 0.8298           | HD 182805 32" away          |
| 2135864872411150720                   | 26665817   | 14.7539    | 14,15             | 1.9827           | object 20" away             |

|                                        |            |         |                |        |                                     |
|----------------------------------------|------------|---------|----------------|--------|-------------------------------------|
| 2149604919464450944                    | 353989024  | 14.9382 | 14-26          | 1.0026 | -                                   |
| 2160276263927353600                    | 233733792  | 12.4555 | 14-17,19-26    | 2.5694 | -                                   |
| 2187704543559462784                    | 1978995005 | 17.7278 | 14,15,16       | 0.1560 | 3 objects within 21"                |
| 2221479066861091840                    | 305721914  | 17.0404 | 16,17,18,24    | 0.2348 | bright object 12" away              |
| 2233741920045058944                    | 417763975  | 15.2579 | 18,19,24       | 2.4500 | object 16" away                     |
| 2234314074112207872                    | 1883795387 | 17.8373 | 14,15,16       | 0.5660 | -                                   |
| 2243609212271977088                    | 467268413  | 16.9912 | 15,16,17,24    | 0.1860 | -                                   |
| 2248022166610310144                    | 1981211186 | 18.1572 | 14-22,24-25    | 0.1158 | -                                   |
| 2265587418916463104                    | 229763894  | 15.0752 | 14-26          | 0.5257 | 3 objects within 21"                |
| 2303705631625361024                    | 397532904  | 12.8886 | 18,19,20,25,26 | 0.4204 | -                                   |
| 333069804659746560                     | 184690162  | 12.8675 | 18             | 0.7554 | crowded field                       |
| 3662392216154435200                    | 392877333  | 12.8925 | 23             | 0.9526 | 2 objects within 53"                |
| 431408849046443264                     | 359433191  | 16.4993 | 17,18,24       | 0.4417 | crowded field                       |
| 4501536260662226560                    | 264050369  | 13.1983 | 26             | 1.5903 | 5 objects within 21"                |
| 4525959987335693056                    | 1684609529 | 16.9125 | 26             | 0.1213 | 3 objects within 21"                |
| 4539247241754918400                    | 337071076  | 13.1383 | 26             | 1.5048 | object 21" away                     |
| 4585910377796460288                    | 84835513   | 13.5448 | 26             | 3.1513 | 4 objects within 21"                |
| 4598451682297980288                    | 310989305  | 14.0091 | 25,26          | 2.4847 | -                                   |
| 562213078769245440                     | 396484881  | 15.7893 | 18,19,25,26    | 0.6073 | 2 objects within 21"                |
| 564551735705888384                     | 609725827  | 16.5793 | 18,19,24,25,26 | 0.1068 | 5 objects within 32"                |
| 893386457796229504                     | 741295718  | 16.7229 | 20             | 1.2233 | <a href="#">Drake et al. (2014)</a> |
| 925671353297509632                     | 29118824   | 13.3735 | 20             | 2.2698 | -                                   |
| 946065369848575872                     | 16600409   | 15.3961 | 20             | 1.1703 | 2 objects within 21"                |
| <b>One asymmetric maximum detected</b> |            |         |                |        |                                     |
| 1328057149815681920                    | 1270359835 | 14.4174 | 24,25          | 1.4561 | very crowded field                  |
| 1328058043172963456                    | 1270366381 | 16.3661 | 24,25          | 0.7509 | very crowded field                  |
| 1360405537821429504                    | 1270837578 | 16.2727 | 25,26          | 0.7026 | very crowded field                  |
| 1360405572181155712                    | 334899908  | 15.7741 | 25,26          | 0.7018 | very crowded field                  |
| 1360408320957344512                    | 1270842390 | 16.5663 | 25,26          | 0.6298 | very crowded field                  |
| 1418837537086251264                    | 1271027428 | 18.9619 | 17,20,23-26    | 0.4771 | -                                   |
| 1702017375296326528                    | 1102619251 | 18.7239 | 14-15,20-22,26 | 4.8500 | -                                   |
| 1705393833770160128                    | 288381009  | 16.4297 | 14-26          | 1.8706 | object 13" away                     |
| 1939433718495541632                    | 177243718  | 13.6373 | 17             | 1.1822 | 3 objects within 21"                |
| 2093534465017435776                    | 258279532  | 10.8904 | 14,26          | 3.9000 | 4 objects within 21"                |
| 2105187256745838080                    | 1716561881 | 17.7428 | 14,26          | 4.3001 | bright object 16" away              |
| 2167371859151731712                    | 195728426  | 16.2172 | 15,16          | 3.1822 | 5 bright objects within 21"         |
| 2198794939398092160                    | 330843247  | 16.2883 | 16,17,24       | 0.6260 | 4 bright objects within 21"         |
| 4534814663708775552                    | 1814743619 | 17.5482 | 14             | 3.1277 | crowded field                       |
| 4607722936142361216                    | 1508465315 | 18.8009 | 25,26          | 0.5967 | 3 objects within 21"                |
| 524799859180542080                     | 54051804   | 14.2380 | 18,24,25       | 2.1242 | 2 bright objects within 21"         |
| <b>Two maxima detected</b>             |            |         |                |        |                                     |
| 1816862670495460352                    | 1943342834 | 18.1102 | 14             | 0.3207 | crowded field                       |
| 1907427033790181248                    | 2003766169 | 18.2384 | 16             | 0.7305 | -                                   |
| 1962740066464303744                    | 2006587293 | 7.5790  | 16             | 2.4021 | V1942 Cyg 1" away                   |
| 1976684313460272128                    | 2010382498 | 16.9980 | 16             | 2.5714 | crowded field                       |
| 1979662924824022528                    | 2011878719 | 16.1120 | 16             | 0.3919 | crowded field                       |

|                     |            |         |       |        |                                             |
|---------------------|------------|---------|-------|--------|---------------------------------------------|
| 2039164989422375168 | 1712800054 | 16.6814 | 14    | 0.8764 | crowded field                               |
| 2100480767163455360 | 121107327  | 16.2609 | 14    | 0.5772 | CV ( <a href="#">Fontaine et al. 2010</a> ) |
| 2242271072260536832 | 229463748  | 13.8202 | 14-26 | 1.2363 | -                                           |
| 2288995609155671936 | 1884532373 | 16.5623 | 14-26 | 0.4107 | -                                           |
| 3974187703469677568 | 156952109  | 13.3871 | 22    | 0.5971 | -                                           |
| 4532553445024997376 | 1813751285 | 18.1596 | 26    | 3.2319 | crowded field                               |
| 4554252723613727872 | 1506996219 | 16.8171 | 25,26 | 0.4738 | 2 objects within 21"                        |
| 498498166646842496  | 310922669  | 11.8079 | 19,26 | 0.5656 | crowded field                               |
| 504667698197248640  | 445526365  | 10.1176 | 18    | 2.0482 | crowded field                               |

One symmetric maximum detected

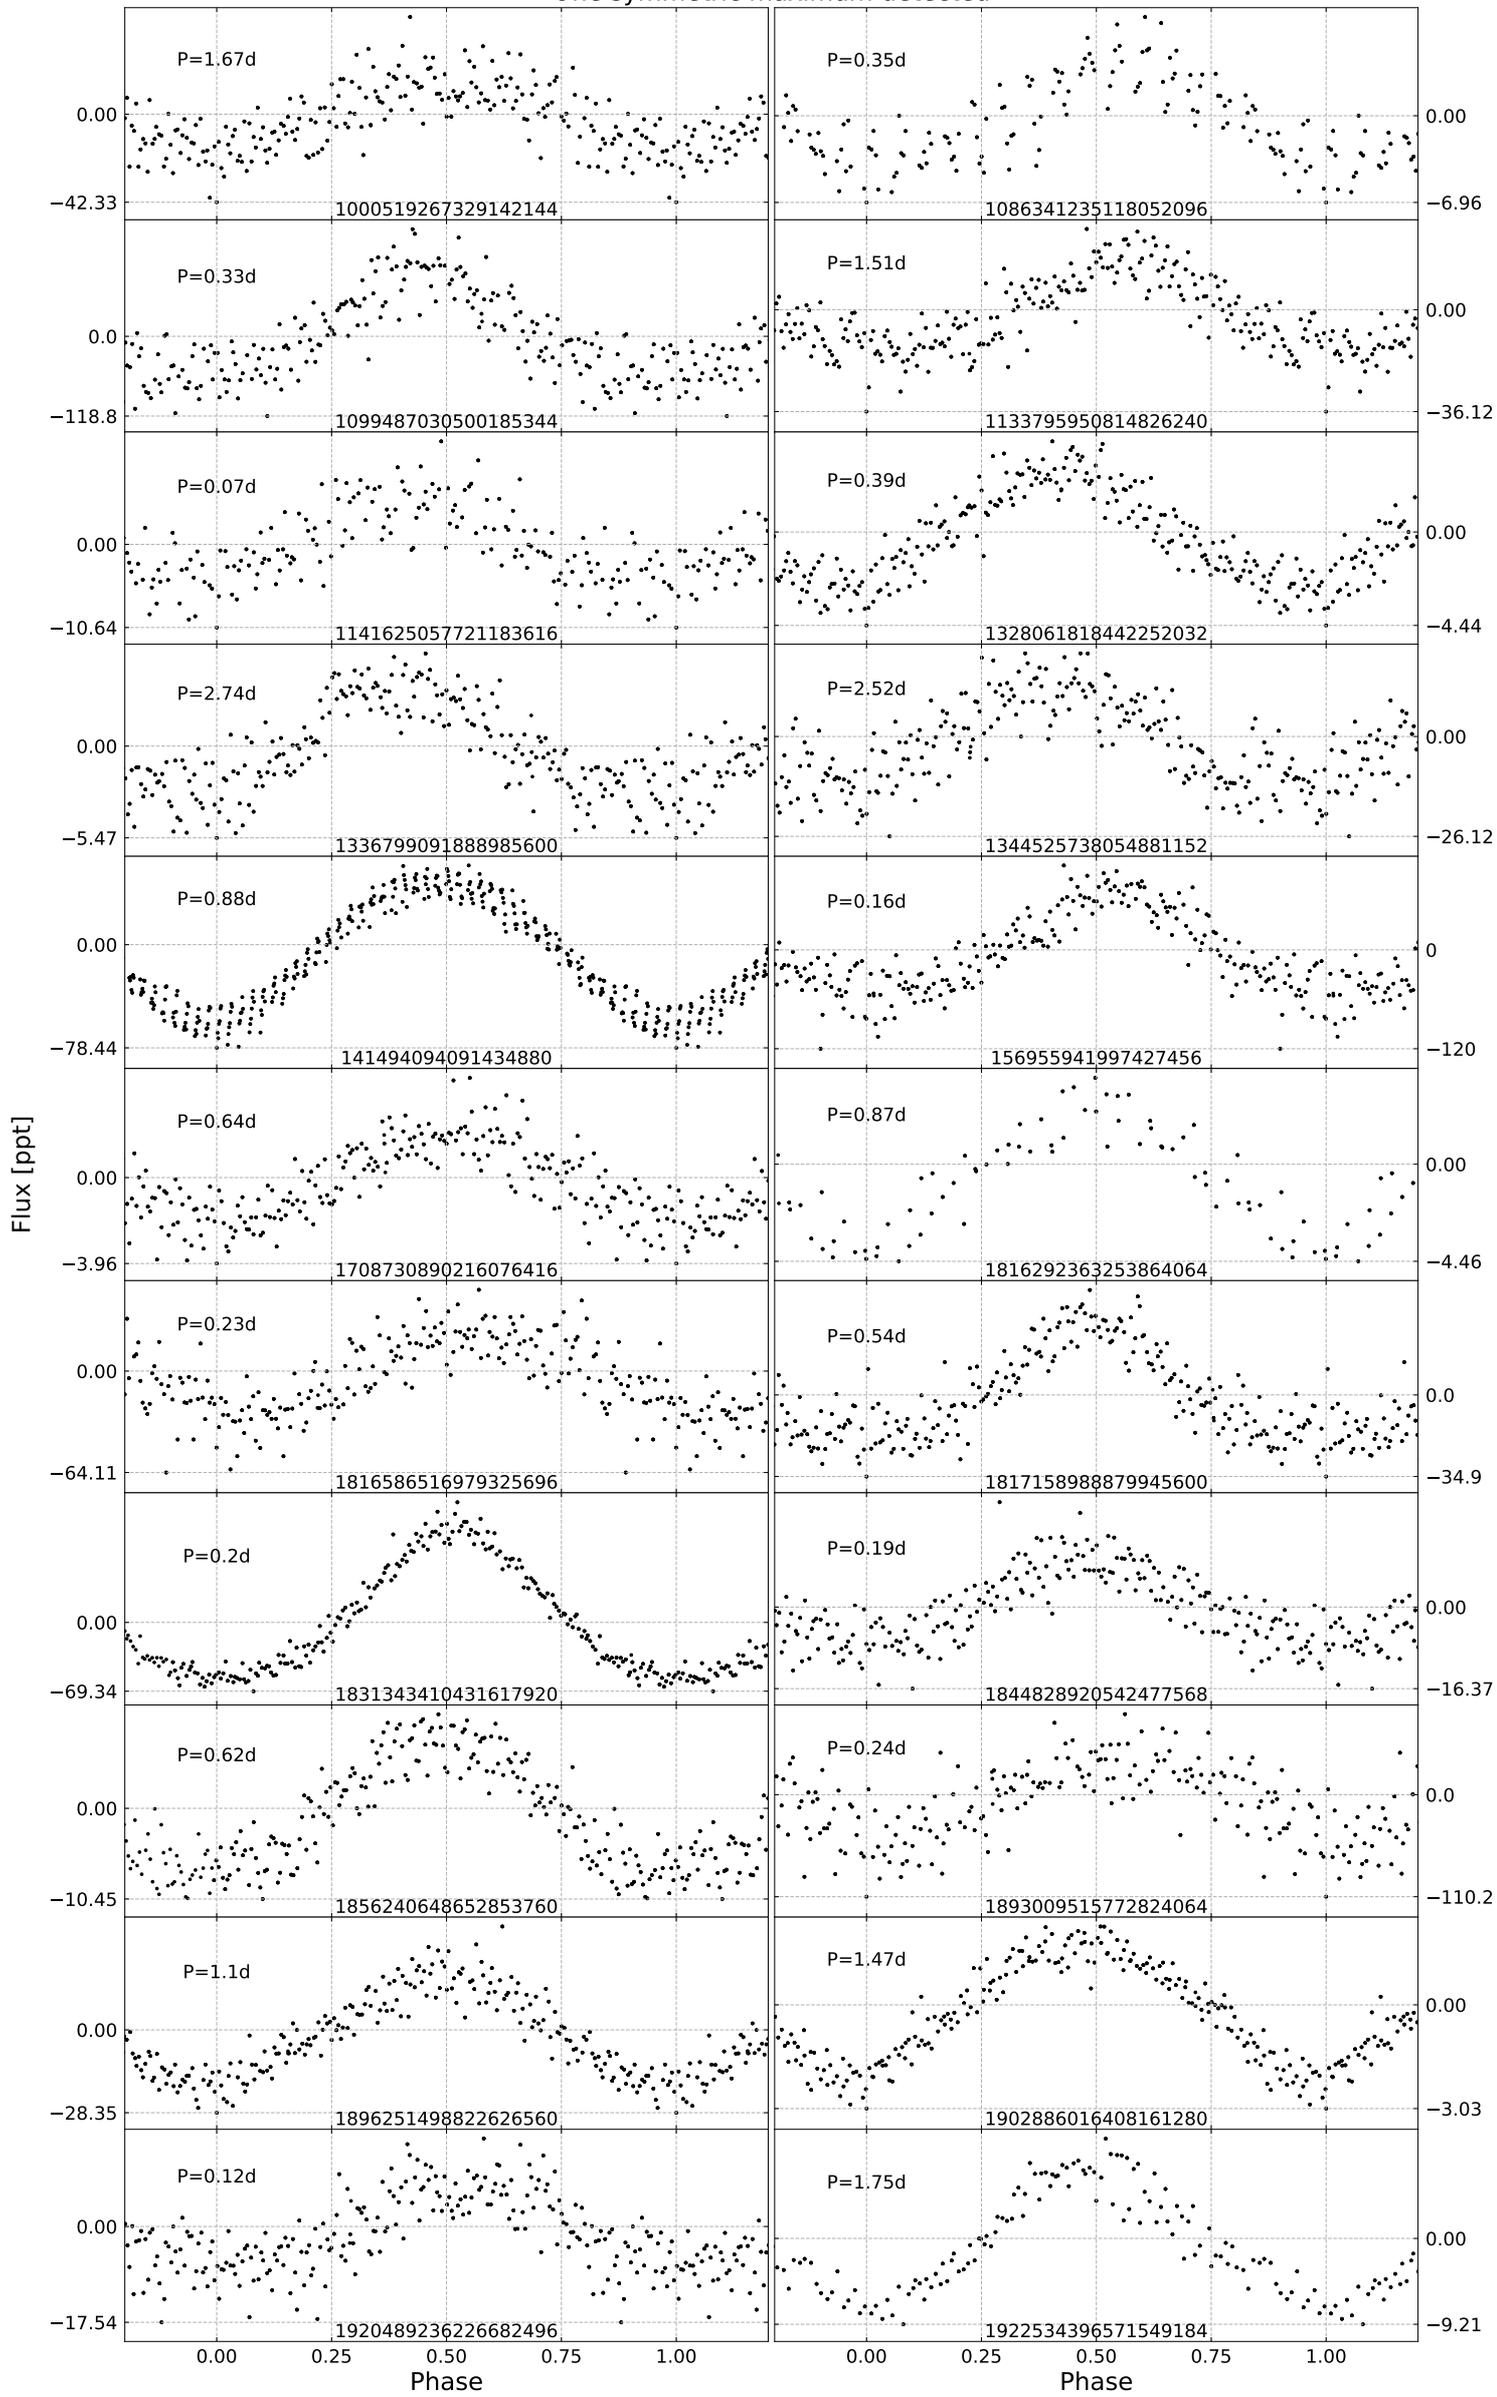

One symmetric maximum detected

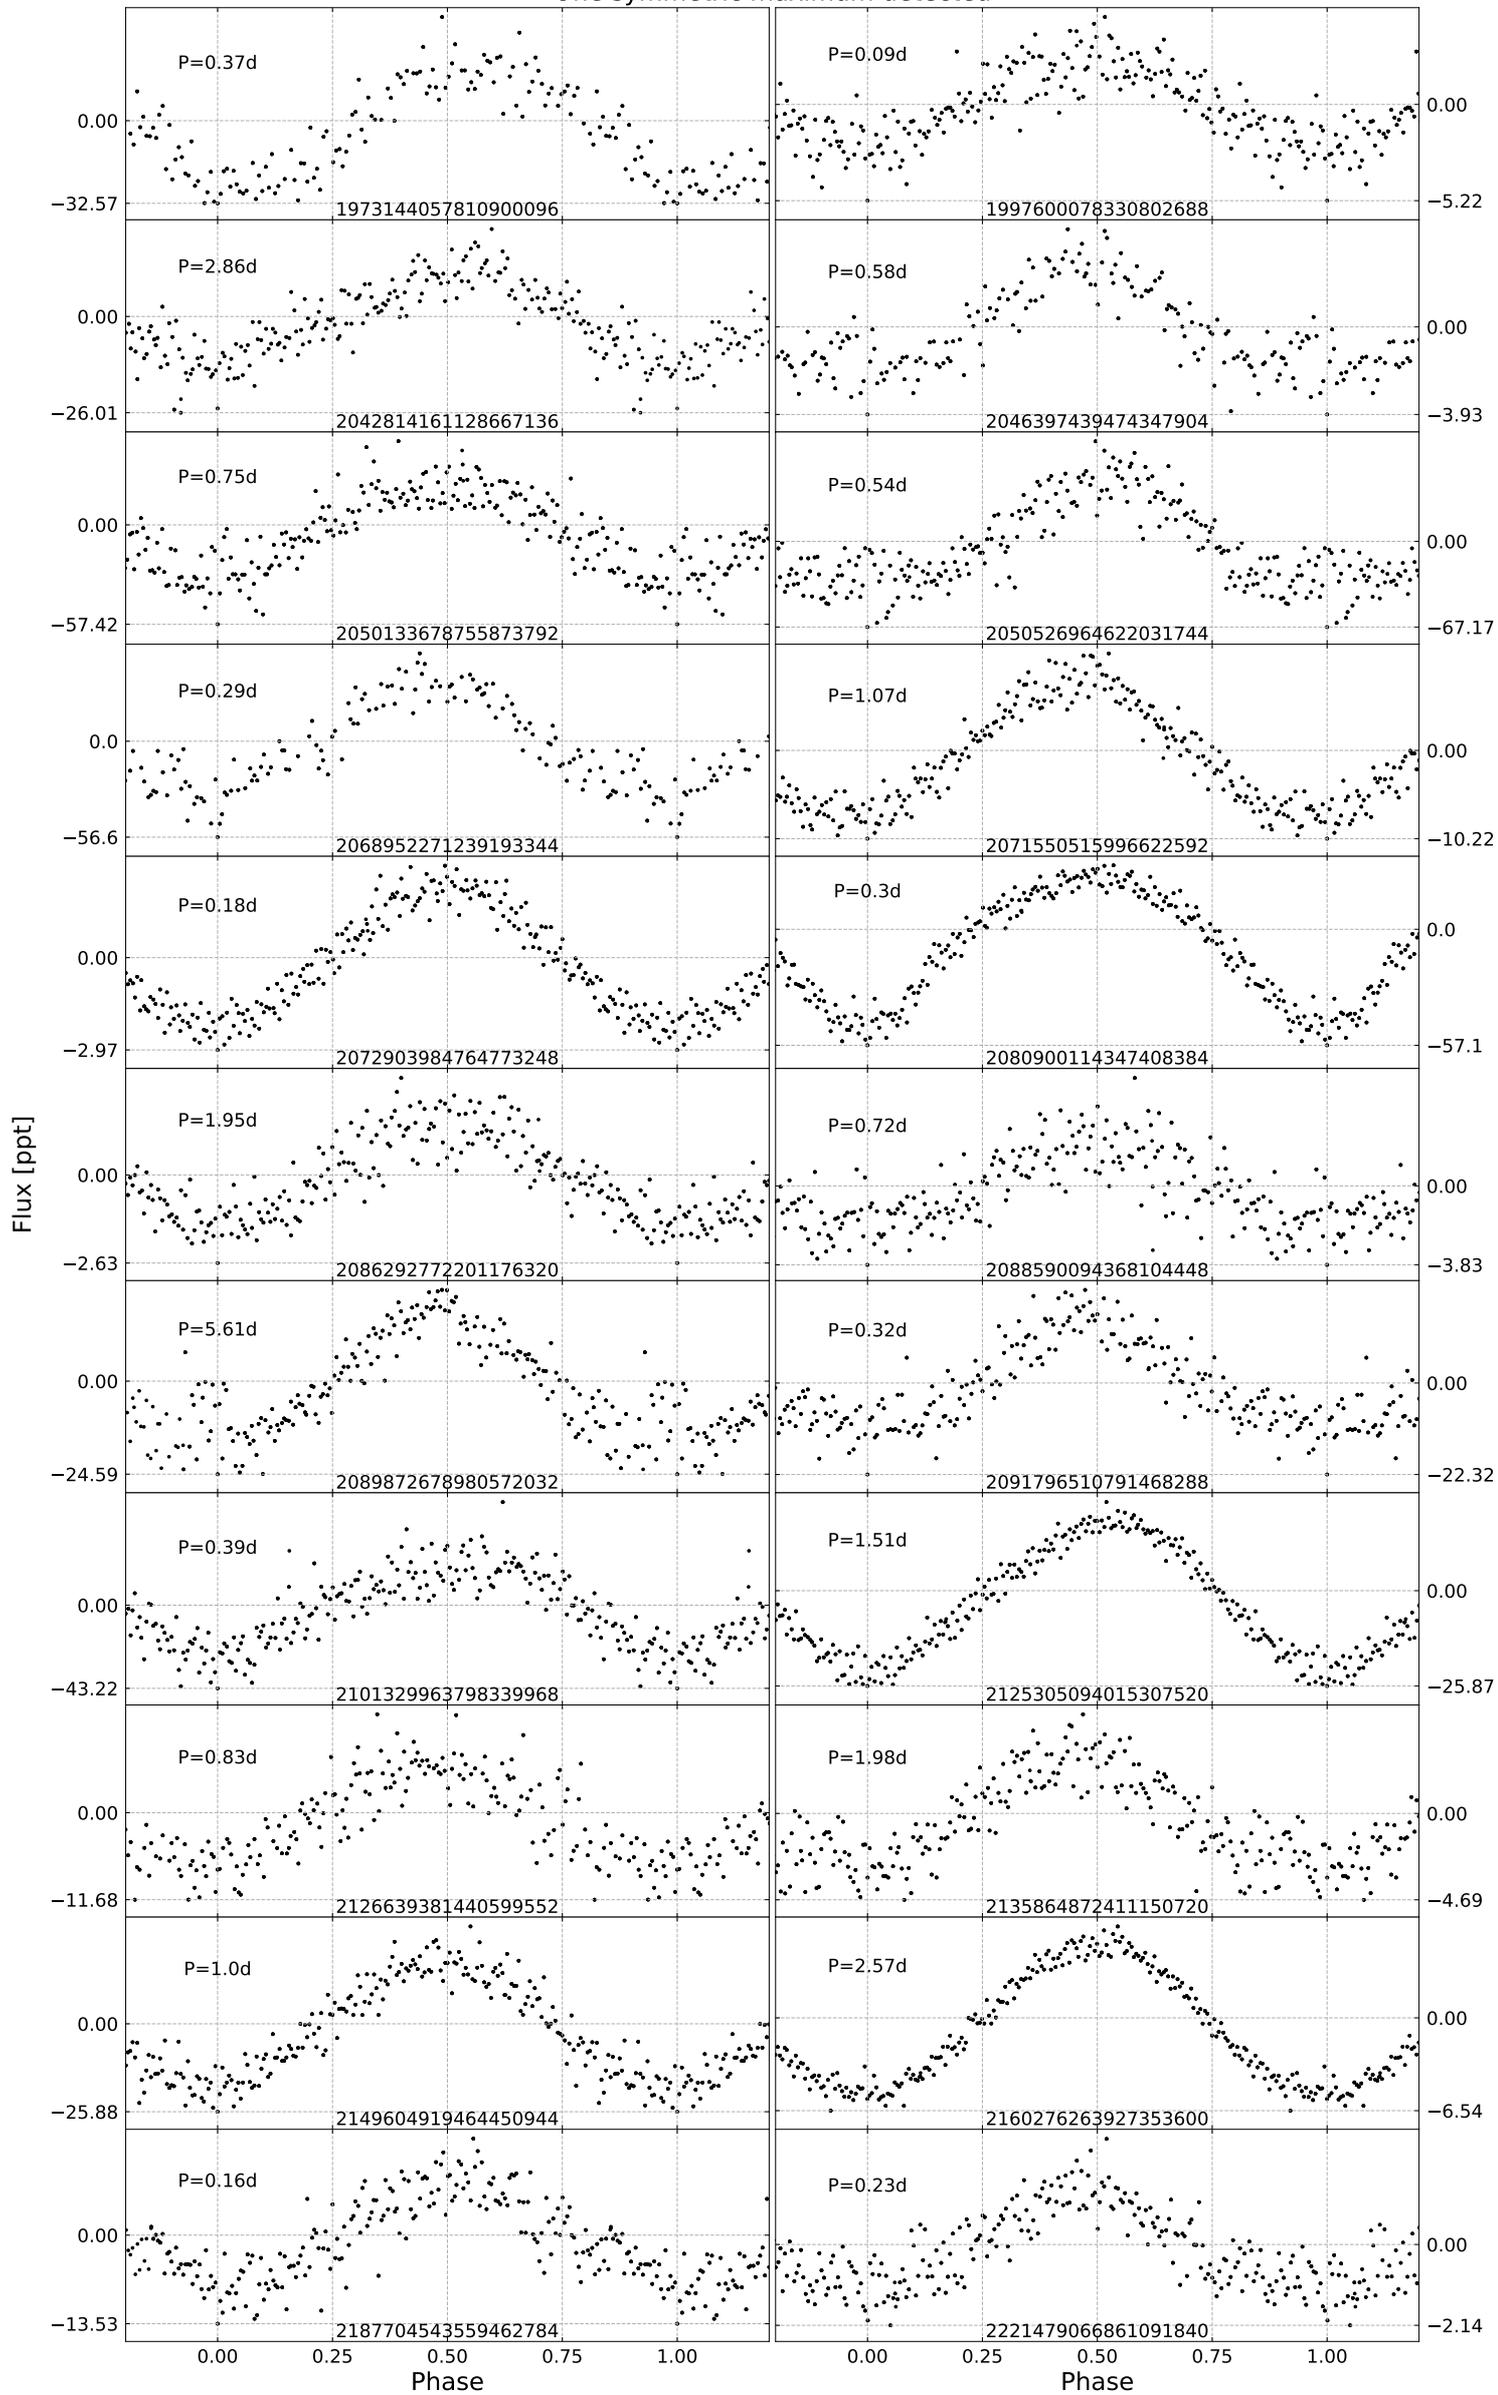

One symmetric maximum detected

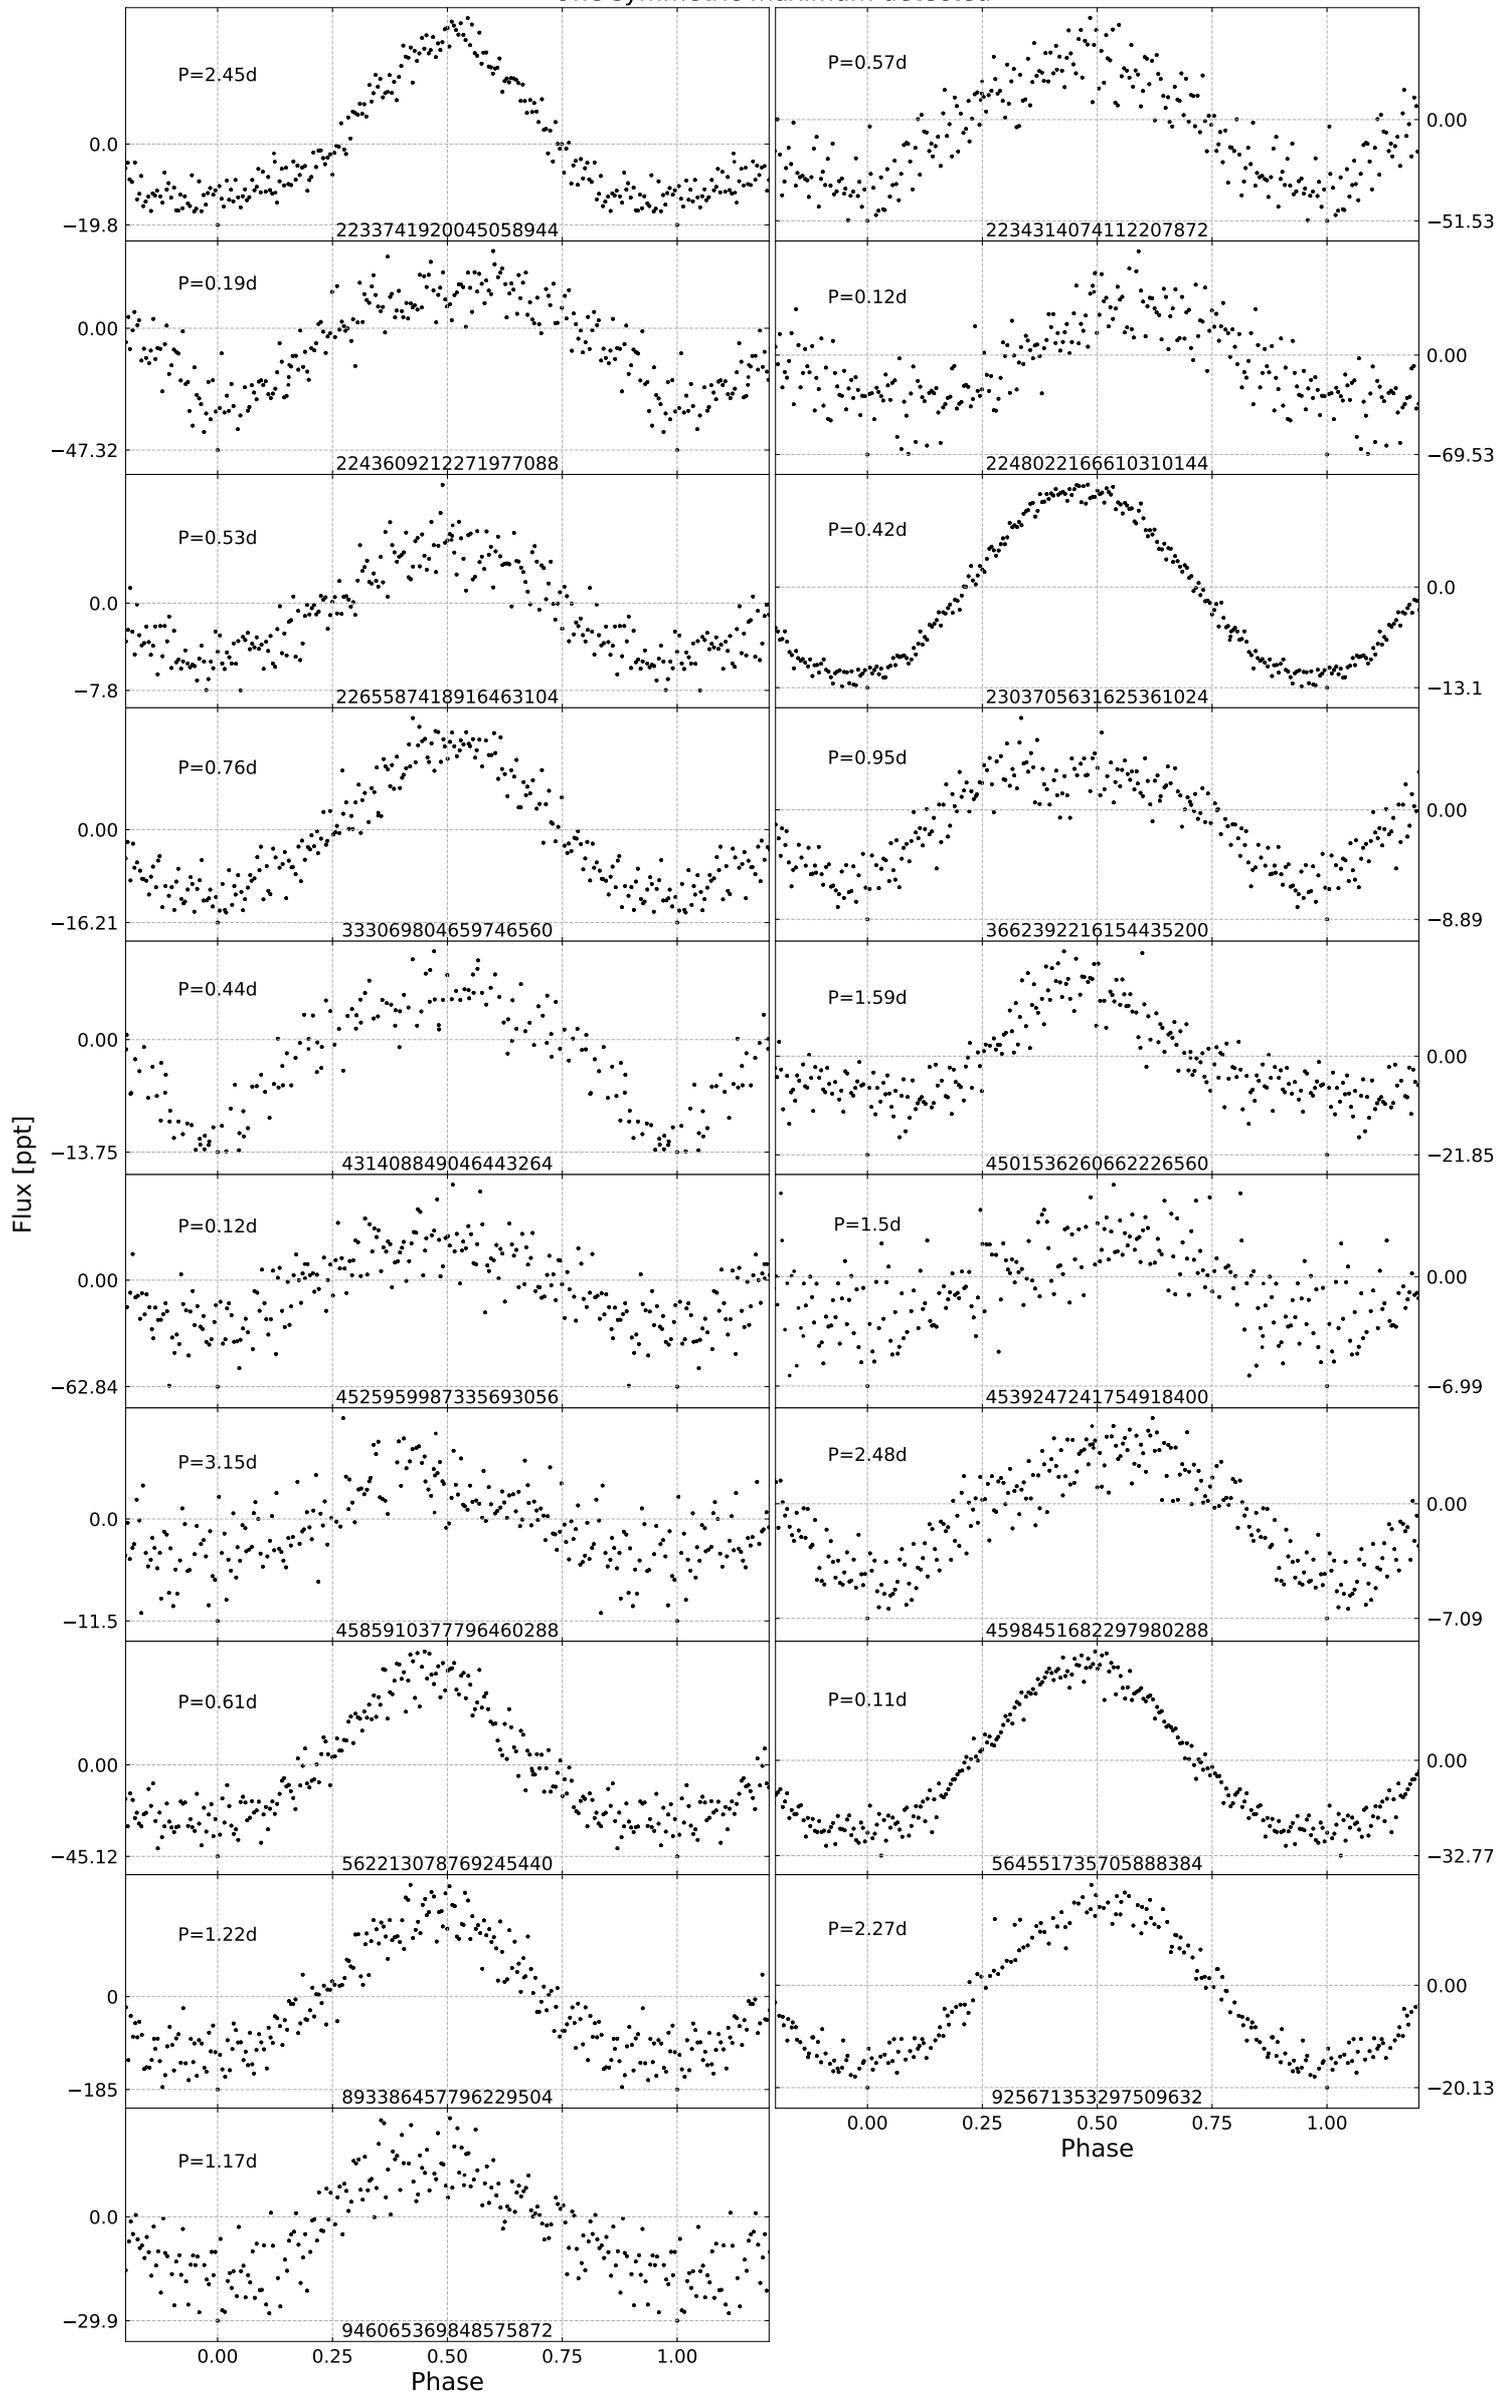

# One asymmetric maximum detected

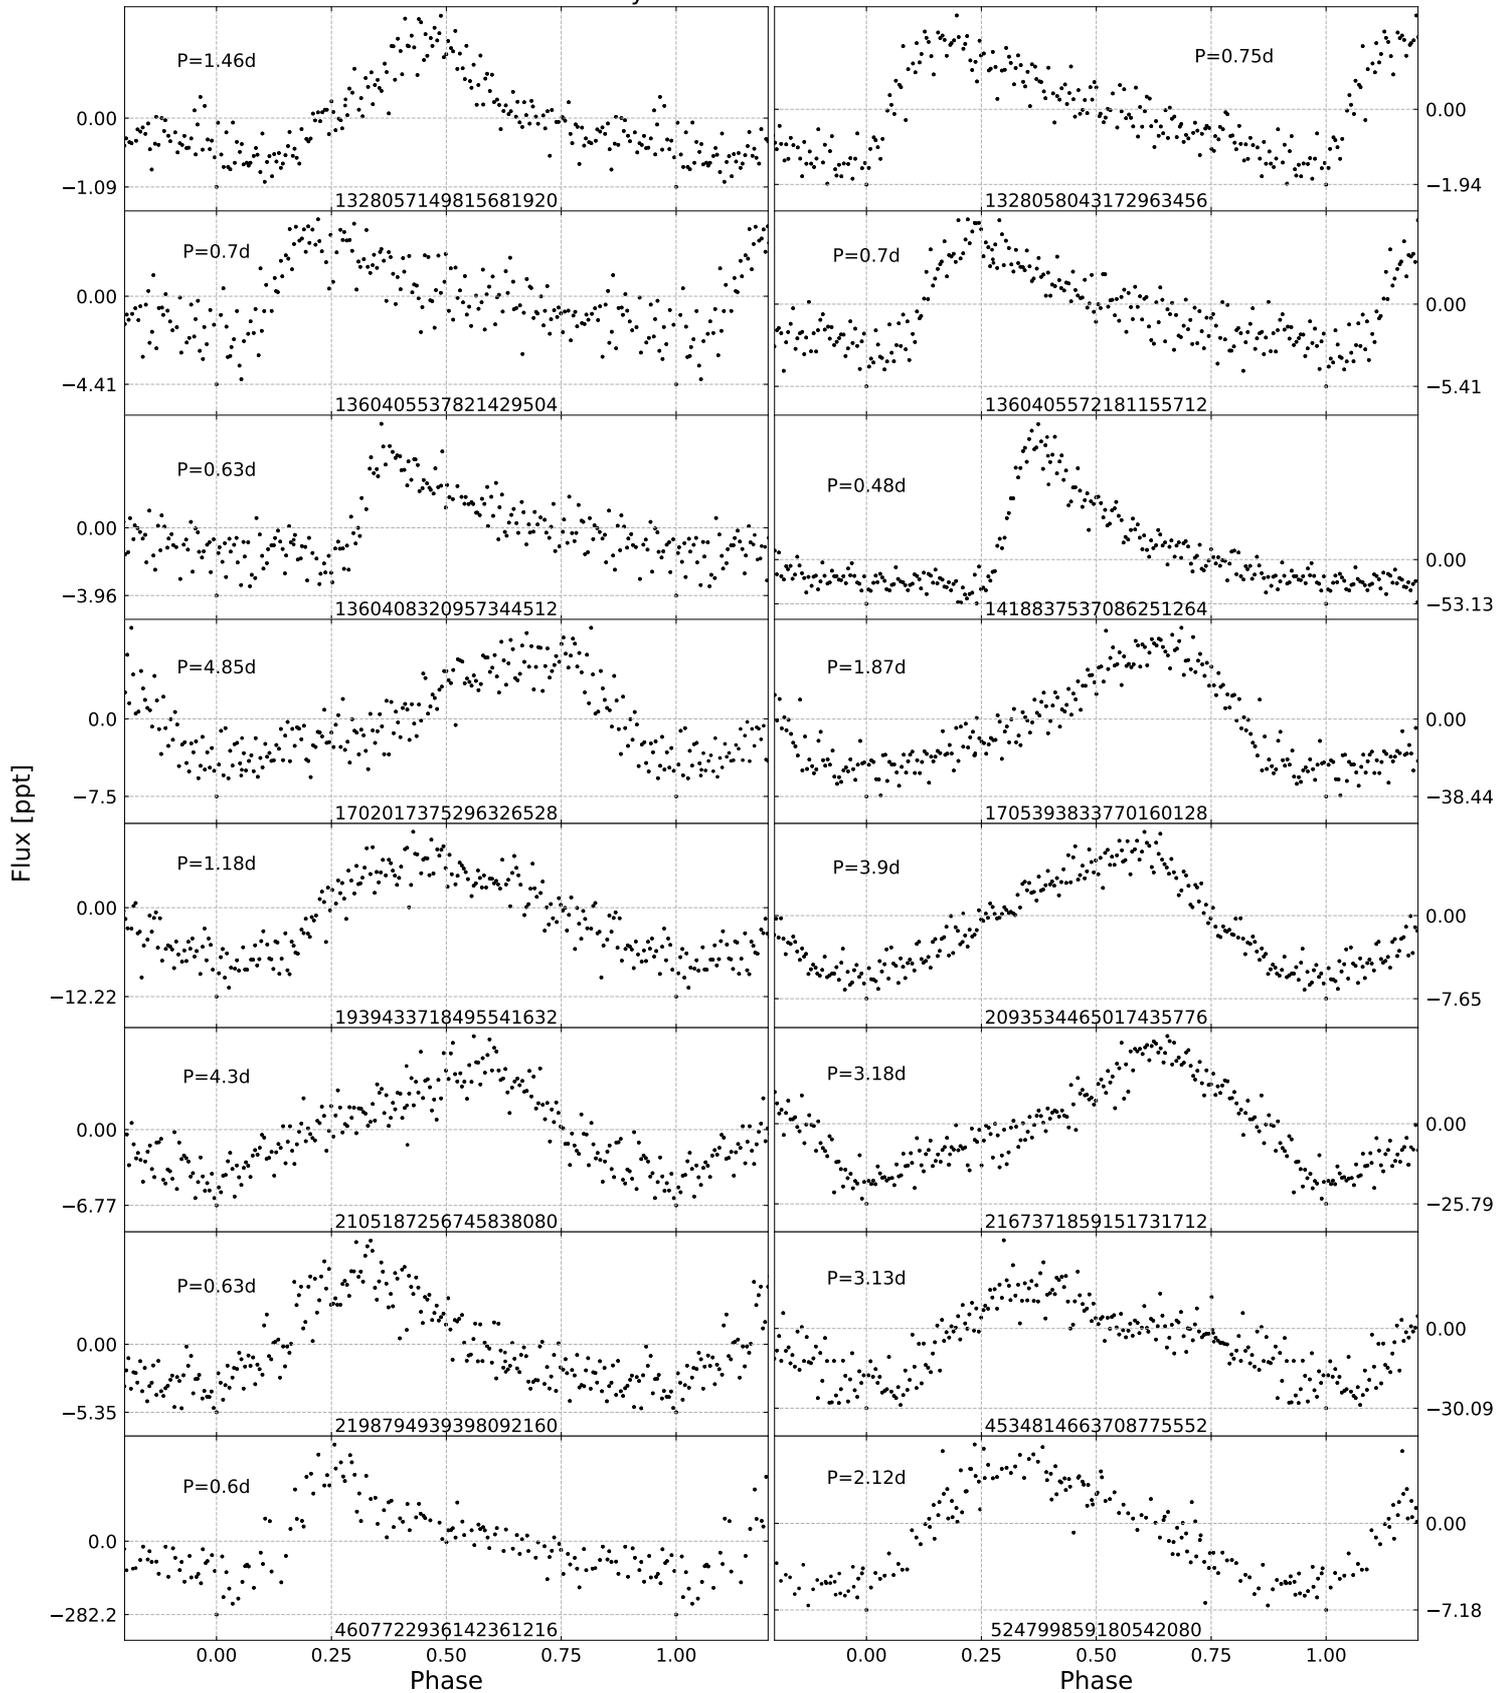

## Two maxima detected

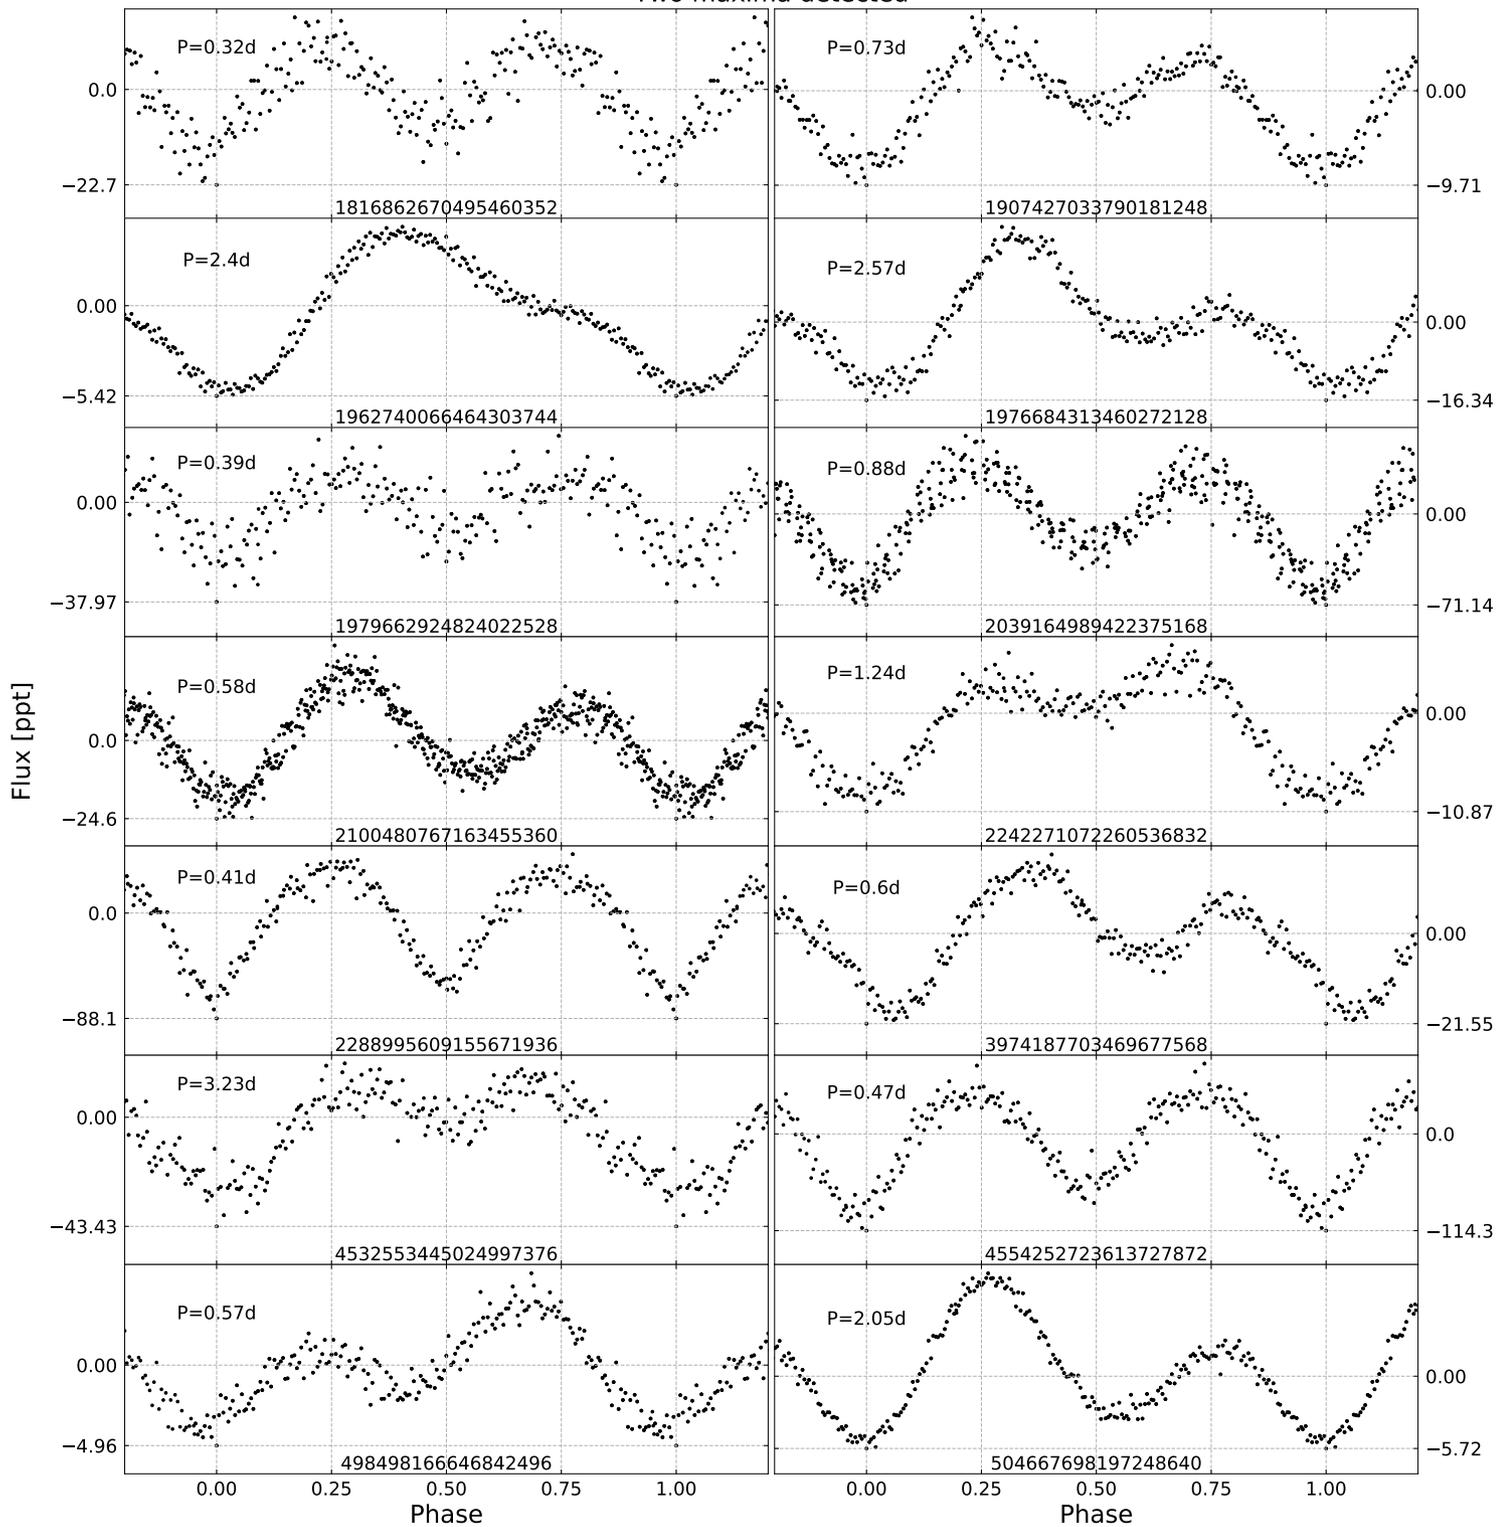

Supplement: Supplementary file 3 [file nospec_phased.pdf]
